# Supplementary material for: MAML and ANIL Provably Learn Representations
Source: arXiv:2202.03483 source file (2023-06-04)
Supplement: Supplementary file 1 [file Appendix_ANIL_new_FS.tex]

\subsection{Finite Samples}
% {\color{blue} 11/1: The proof is for FO-MAML under assumption that $\|\mathbf{w}_t\|_2$ is bounded. The analysis for ANIL that differs from FO-ANIL is added in blue. For both FO-ANIL and ANIL it only remains to bound $\|\mathbf{w}_t\|$. But it is not clear how to do this because the $\delta$'s are not summable.}

% Let $\mu_{\ast,t}^2 = \sigma_{\min}\left(\frac{1}{n} \sum_{i=1}^n \mathbf{w}_{\ast,t,i} \mathbf{w}_{\ast,t,i}^\top\right)$ and $L_{\ast,t}^2 = \sigma_{\max}\left(\frac{1}{n} \sum_{i=1}^n \mathbf{w}_{\ast,t,i} \mathbf{w}_{\ast,t,i}^\top\right)$.
% Let $A \coloneqq \cap_{t=1}^T \left\{\mu_{\ast,t}^2 \geq \mu_\ast^2 \text{ and } L_{\ast, t}^2 \leq L_\ast^2\right\}$. By Lemma \ref{lem:task_diversity}, $P(A) \geq 1 - 2 T e^{-\gamma^2}$.

% Let $\mathbf{\Sigma}_{t,i}^{out} \coloneqq \frac{1}{m_{out}} \sum_{j=1}^{m_{out}} \mathbf{x}_{t,i,j}^{out}(\mathbf{x}_{t,i,j}^{out})^\top$, $\mathbf{\Sigma}_{t,i}^{in} \coloneqq \frac{1}{m_{in}} \sum_{j=1}^{m_{in}} \mathbf{x}_{t,i,j}^{in}(\mathbf{x}_{t,i,j}^{in})^\top$,  $\mathbf{X}_{t,i}^{out} = [\mathbf{x}_{t,i,1}^{out}, \dots, \mathbf{x}_{t,i,m_{out}}^{out}]^\top$, $\mathbf{X}_{t,i}^{in} = [\mathbf{x}_{t,i,1}^{in}, \dots, \mathbf{x}_{t,n,m_{in}}^{in}]^\top$, $\mathbf{z}_{t,i}^{out} = [z_{t,i,1},\dots, z_{t,i,m_{out}}]$ and  $\mathbf{z}_{t,i}^{in} = [z_{t,i,1},\dots, z_{t,i,m_{in}}]$.

The inner loop update for the head of the $i$-th task on iteration $t$ is given by:
\begin{align}
    \mathbf{w}_{t,i} %&= \mathbf{w}_t - \alpha \mathbf{B}_t ^\top \sum_{j=1}^{m_{in}}\mathbf{x}_{i,j}\mathbf{x}_{i,j}^\top \mathbf{B}_t \mathbf{{w}}_t  + \alpha \mathbf{B}_t ^\top \frac{1}{m_{in}}\sum_{j=1}^{m_{in}}\mathbf{x}_{i,j}\mathbf{x}_{i,j}^\top \mathbf{\hat{B}}_\ast \mathbf{{w}}_{\ast,i} \nonumber \\
    &= \mathbf{w}_t - \alpha \nabla_{\mathbf{w}} \hat{\mathcal{L}}_i(\mathbf{B}_t, \mathbf{w}_t, \mathcal{D}_{i}^{in}) \nonumber \\
    &=  (\mathbf{I}_k- \alpha\mathbf{B}_t ^\top \mathbf{\Sigma}_{t,i}^{in} \mathbf{B}_t )\mathbf{{w}}_t + \alpha \mathbf{B}_t ^\top \mathbf{\Sigma}_{t,i}^{in} \mathbf{\hat{B}}_\ast\mathbf{{w}}_{\ast,t,i} + \frac{\alpha}{m_{in}} \mathbf{B}_t ^\top (\mathbf{X}_{t,i}^{in})^\top \mathbf{z}_{t,i}^{in}. \label{upd_head_anil}
\end{align}
The outer loop updates for the head and representation are:
\begin{align}
\mathbf{w}_{t+1} &= \mathbf{w}_t - \frac{\beta}{n}\sum_{i=1}^n \nabla_{\mathbf{w}} \hat{\mathcal{L}}_i(\mathbf{B}_t , \mathbf{w}_{t,i}) \nonumber \\
&=  \mathbf{{w}}_{t} - \frac{\beta}{n}\sum_{i=1}^{n}\mathbf{B}_t ^\top \mathbf{\Sigma}_{t,i}^{out} \mathbf{B}_t \mathbf{{w}}_{t,i} + \frac{\beta}{n}\sum_{i=1}^n \mathbf{B}_t ^\top \mathbf{\Sigma}_{t,i}^{out} \mathbf{\hat{B}}_\ast\mathbf{{w}}_{\ast,i} + \frac{\beta}{n m_{out}}\sum_{i=1}^n \mathbf{B}_t ^\top (\mathbf{X}_{t,i}^{out})^\top\mathbf{z}_{t,i}^{out} \label{upd_head_out_anil} \\
    \mathbf{{B}}_{t+1} &= \mathbf{B}_t  - \frac{\beta}{n}\sum_{i=1}^n \nabla_{\mathbf{B}} \hat{\mathcal{L}}_i(\mathbf{B}_t , \mathbf{w}_{t,i}) \nonumber \\
    &= \mathbf{{B}}_t  - \frac{\beta}{n}\sum_{i=1}^n  \mathbf{\Sigma}_{t,i}^{out} \mathbf{B}_t  \mathbf{w}_{t,i}\mathbf{w}_{t,i}^\top + \frac{\beta}{n } \sum_{i=1}^n \mathbf{\Sigma}_{t,i}^{out} \mathbf{\hat{B}}_\ast\mathbf{w}_{\ast,t,i} \mathbf{w}_{t,i}^\top  + \frac{\beta}{nm_{out}}\sum_{i=1}^n(\mathbf{X}^{out}_{t,i})^\top \mathbf{z}^{out}_{t,i}\mathbf{w}_{t,i}^\top  \label{upd_rep_anil}
    % &= \mathbf{B}_t \left(\mathbf{I} - \frac{\beta}{n}\sum_{i=1}^n \mathbf{w}_{t,i}\mathbf{w}_{t,i}^\top\right) + \mathbf{\hat{B}}_\ast\left(\frac{\beta}{n} \sum_{i=1}^n \mathbf{w}_{\ast,t,i} \mathbf{w}_{t,i}^\top \right) \nonumber \\
    % &\quad + \frac{\beta}{n} \sum_{i=1}^n \left(\mathbf{I}_d - \frac{1}{m_{out}}\sum_{j=1}^{m_{out}} \mathbf{x}_{i,j}\mathbf{x}_{i,j}^\top \right) \mathbf{B}_t  \mathbf{w}_{t,i}\mathbf{w}_{t,i}^\top  - \frac{\beta}{n} \sum_{i=1}^n \left(\mathbf{I}_d - \frac{1}{m_{out}}\sum_{j=1}^{m_{out}} \mathbf{x}_{i,j}\mathbf{x}_{i,j}^\top \right) \mathbf{\hat{B}}_\ast \mathbf{w}_{\ast,t,i}\mathbf{w}_{t,i}^\top
    % \mathbf{\hat{B}}_{t+1}, \mathbf{R}_{t+1} &= \text{QR}(\mathbf{\bar{B}}_{t+1})
\end{align}
We can write the updates $\mathbf{w}_{t,i}, \mathbf{w}_{t+1},$ and $\mathbf{B}_{t+1}$ as the updates from the population case plus perturbation terms due to having finite samples, as follows:
% The update for $\mathbf{B}$ is:
\begin{align}
\mathbf{w}_{t,i} &= (\mathbf{I}_k-\alpha\mathbf{B}_t^\top \mathbf{B}_t)\mathbf{{w}}_t + \alpha\mathbf{B}_t ^\top \mathbf{\hat{B}}_\ast\mathbf{{w}}_{\ast,t,i}  \nonumber \\
&\quad + \alpha (\mathbf{B}_t^\top\mathbf{B}_t - \mathbf{B}_t^\top\mathbf{\Sigma}_{t,i}^{in} \mathbf{B}_t )  \mathbf{{w}}_{t} - \alpha (\mathbf{B}_t ^\top \mathbf{\hat{B}}_\ast - \mathbf{B}_t ^\top  \mathbf{\Sigma}_{t,i}^{in} \mathbf{\hat{B}}_\ast) \mathbf{{w}}_{\ast,t,i}  +  \frac{\alpha}{m_{in}} \mathbf{B}_t ^\top (\mathbf{X}_{t,i}^{in})^\top \mathbf{z}_{t,i}^{in} \label{anil_e_wi}\\
\mathbf{w}_{t+1} &= \mathbf{{w}}_{t} -\frac{\beta}{n}\sum_{i=1}^n \mathbf{B}_t^\top\mathbf{B}_t \mathbf{{w}}_{t,i} + \frac{\beta}{n}\sum_{i=1}^n  \mathbf{B}_t ^\top \mathbf{\hat{B}}_\ast\mathbf{{w}}_{\ast,t,i}  \nonumber \\
&\quad + \frac{\beta}{n}\sum_{i=1}^n (\mathbf{B}_t^\top\mathbf{B}_t - \mathbf{B}_t^\top\mathbf{\Sigma}_{t,i}^{out} \mathbf{B}_t )  \mathbf{{w}}_{t,i} - \frac{\beta}{n}\sum_{i=1}^n  (\mathbf{B}_t ^\top \mathbf{\hat{B}}_\ast - \mathbf{B}_t ^\top  \mathbf{\Sigma}_{t,i}^{out} \mathbf{\hat{B}}_\ast) \mathbf{{w}}_{\ast,t,i}\nonumber \\
&\quad +  \frac{\beta}{nm_{out}} \sum_{i=1}^n \mathbf{B}_t ^\top (\mathbf{X}_{t,i}^{out})^\top \mathbf{z}_{t,i}^{out} \label{anil_e_w}\\
    \mathbf{B}_{t+1} &= \mathbf{{B}}_t\left(\mathbf{I}_k - \frac{\beta}{n}\sum_{i=1}^n \mathbf{w}_{t,i}\mathbf{w}_{t,i}^\top\right) + \mathbf{\hat{B}}_\ast\left(\frac{\beta}{n} \sum_{i=1}^n \mathbf{w}_{\ast,t,i} \mathbf{w}_{t,i}^\top \right) - \beta \alpha  \lambda \mathbf{B}_t (\alpha \mathbf{B}_t^\top \mathbf{B}_t - \mathbf{I}_k) \nonumber \\
    &\quad + \frac{\beta}{n} \sum_{i=1}^n \left(\mathbf{I}_d - \mathbf{\Sigma}_{t,i}^{out}\right) \left(\mathbf{B}_t  \mathbf{w}_{t,i} - \mathbf{\hat{B}}_\ast \mathbf{w}_{\ast,t,i}\right)\mathbf{w}_{t,i}^\top  + \frac{\beta}{n m_{out}}\sum_{i=1}^n(\mathbf{X}^{out}_{t,i})^\top \mathbf{z}^{out}_{t,i}\mathbf{w}_{t,i}^\top  \label{anil_e_b}
\end{align}

{
% \color{blue}
We can write the updates $\mathbf{w}_{t,i}, \mathbf{w}_{t+1},$ and $\mathbf{B}_{t+1}$ as the updates from the population case plus perturbation terms due to having finite samples, as follows:
\begin{align}
    \mathbf{w}_{t+1} &= \mathbf{{w}}_{t} - (\mathbf{I}_k - \alpha\mathbf{B}_t^\top\mathbf{B}_t )\frac{\beta}{n}\sum_{i=1}^n (\mathbf{B}_t^\top\mathbf{B}_t  \mathbf{{w}}_{t,i} -  \mathbf{B}_t^\top \mathbf{\hat{B}}_\ast\mathbf{{w}}_{\ast,t,i})  \nonumber \\
&\quad + (\mathbf{I}_k - \alpha\mathbf{B}_t^\top\mathbf{B}_t )\frac{\beta}{n}\sum_{i=1}^n (\mathbf{B}_t^\top\mathbf{B}_t - \mathbf{B}_t ^\top\mathbf{\Sigma}_{t,i}^{out} \mathbf{B}_t )  \mathbf{{w}}_{t,i} - (\mathbf{I}_k - \alpha\mathbf{B}_t^\top\mathbf{B}_t )\frac{\beta}{n}\sum_{i=1}^n  (\mathbf{B}_t ^\top \mathbf{\hat{B}}_\ast - \mathbf{B}_t ^\top  \mathbf{\Sigma}_{t,i}^{out} \mathbf{\hat{B}}_\ast) \mathbf{{w}}_{\ast,t,i}\nonumber \\
&\quad +   (\mathbf{I}_k - \alpha \mathbf{B}_t^\top\mathbf{B}_t)\frac{\beta}{nm_{out}} \sum_{i=1}^n \mathbf{B}_t ^\top (\mathbf{X}_{t,i}^{out})^\top \mathbf{z}_{t,i}^{out} \nonumber  \\
&\quad - \alpha \frac{\beta}{n}\sum_{i=1}^n(\mathbf{B}_t^\top\mathbf{B}_t - \mathbf{B}_t^\top\mathbf{\Sigma}_{t,i}^{out}\mathbf{B}_t ) (\mathbf{B}_t^\top\mathbf{B}_t  \mathbf{{w}}_{t,i} -  \mathbf{B}_t^\top \mathbf{\hat{B}}_\ast\mathbf{{w}}_{\ast,t,i})  \nonumber \\
&\quad + \alpha \frac{\beta}{n}\sum_{i=1}^n (\mathbf{B}_t^\top\mathbf{B}_t - \mathbf{B}_t^\top\mathbf{\Sigma}_{t,i}^{out}\mathbf{B}_t )(\mathbf{B}_t^\top\mathbf{B}_t - \mathbf{B}_t ^\top\mathbf{\Sigma}_{t,i}^{out} \mathbf{B}_t )  \mathbf{{w}}_{t,i} \nonumber \\
&\quad + \alpha \frac{\beta}{n}\sum_{i=1}^n  (\mathbf{B}_t^\top\mathbf{B}_t - \mathbf{B}_t^\top\mathbf{\Sigma}_{t,i}^{out}\mathbf{B}_t )(\mathbf{B}_t ^\top \mathbf{\hat{B}}_\ast - \mathbf{B}_t ^\top  \mathbf{\Sigma}_{t,i}^{out} \mathbf{\hat{B}}_\ast) \mathbf{{w}}_{\ast,t,i}\nonumber \\
&\quad +   \alpha\frac{\beta}{nm_{out}} \sum_{i=1}^n (\mathbf{B}_t^\top\mathbf{B}_t - \mathbf{B}_t^\top\mathbf{\Sigma}_{t,i}^{out}\mathbf{B}_t ) \mathbf{B}_t ^\top (\mathbf{X}_{t,i}^{out})^\top \mathbf{z}_{t,i}^{out} \nonumber  \\
&\quad + \alpha (\mathbf{B}_t^\top\mathbf{B}_t - \mathbf{B}_t^\top\mathbf{\Sigma}_{t,i}^{out}\mathbf{B}_t)\frac{\beta}{nm_{out}} \sum_{i=1}^n \mathbf{B}_t ^\top (\mathbf{X}_{t,i}^{out})^\top \mathbf{z}_{t,i}^{out}   \label{anil_e_w_exact}\\
    \mathbf{B}_{t+1} &= \mathbf{{B}}_t\left(\mathbf{I}_k - \frac{\beta}{n}\sum_{i=1}^n \mathbf{w}_{t,i}\mathbf{w}_{t,i}^\top\right) + \mathbf{\hat{B}}_\ast\left(\frac{\beta}{n} \sum_{i=1}^n \mathbf{w}_{\ast,t,i} \mathbf{w}_{t,i}^\top \right) - \beta \alpha  \lambda \mathbf{B}_t (\alpha \mathbf{B}_t^\top \mathbf{B}_t - \mathbf{I}_k) \nonumber \\
    &\quad + \frac{\beta}{n} \sum_{i=1}^n \left(\mathbf{I}_d - \mathbf{\Sigma}_{t,i}^{out}\right) \left(\mathbf{B}_t  \mathbf{w}_{t,i} - \mathbf{\hat{B}}_\ast \mathbf{w}_{\ast,t,i}\right)\mathbf{w}_{t,i}^\top  + \frac{\beta}{n m_{out}}\sum_{i=1}^n(\mathbf{X}^{out}_{t,i})^\top \mathbf{z}^{out}_{t,i}\mathbf{w}_{t,i}^\top  \label{anil_e_b_exact}
\end{align}
}

First we define the   following parameters which we will use throughout the proof:
\begin{definition}
\begin{itemize}
    \item $L_\ast \coloneqq 1 + C\frac{\sqrt{k} + \sqrt{\log(T)}}{\sqrt{n}}$. 
    \item $\mu_\ast \coloneqq 1 - C\frac{\sqrt{k} + \sqrt{\log(T)}}{\sqrt{n}}$.
    \item $L_{\max} =\sqrt{k + \max(\sqrt{c_{\max}k\log(nT)}, c_{\max}\log(nT))}$.
    \item $\delta_{in} \coloneqq c_{in}\frac{\sqrt{k}+ 10 \sqrt{\log(n)}}{\sqrt{m_{in}}}$ for some absolute constant $c_{in}$. 
    \item $\delta_{out,k} = c_{out,k}\frac{\sqrt{k}+10\log(n)}{\sqrt{m_{out}}}$
    \item $\delta_{out,n} = c_{out,n}\frac{\sqrt{d}}{\sqrt{n m_{out}}}$ for some absolute constant $c_{out}$.
    \item $\delta_{out,n}' = c_{out,n}'\frac{\sqrt{k}}{\sqrt{n m_{out}}}$ for some absolute constant $c_{out}'$.
\end{itemize}
\end{definition}

% \begin{lemma}
% Let $\alpha=1$. With high probability, for any $t \in [T]$, $\|\mathbf{w}_t\|_2 \leq 1 + f(k,n, \log(T))$.
% \end{lemma}
% \begin{proof}
% Note that for ANIL with $\alpha=1$, the sequence $\{\mathbf{w}_t\}_t$ is a symmetric random walk in $\mathbb{R}^k$.
% \end{proof}

\begin{lemma}\label{lem:w_anil_fs}
For any $t$, suppose that the events
\begin{align}
A_2(s) &\coloneqq \{\| \mathbf{I}_k-\alpha \mathbf{B}_s^\top \mathbf{B}_s  \|_2 \leq (1 - 0.5 \beta E_0 \mu_\ast^2  + 5 \beta \sqrt{\alpha} L_{\ast}^2)\|\mathbf{I}_k - \alpha \mathbf{B}_{s-1}^\top \mathbf{B}_{s-1} \|_2 \nonumber \\
 &\quad\quad \quad \quad \quad \quad \quad \quad \quad \quad  + 10 \alpha^2 \beta^2 L_\ast^4 \dist_{s-1}^2\},
\nonumber \\
A_3(s) &\coloneqq \{\| \mathbf{I}_k-\alpha \mathbf{B}_s^\top \mathbf{B}_s  \|_2 \leq \tau\}, \nonumber \\
 A_5(s) &\coloneqq \{\dist(\mathbf{B}_s, \mathbf{\hat{B}}_\ast) \leq \left(1 - \beta \left(0.5 \alpha E_0 \mu_\ast^2 - 3  \tau_2 \sqrt{\alpha} L_\ast^2  \right) \right)^{s-1}\}
 \end{align}
hold for all $s\in[t]$.
Then
\begin{align}
    \|\mathbf{w}_{t+1}\|_2 \leq \sqrt{\tau_1}
\end{align}
with probability at least  .
\end{lemma}

\begin{proof}
The proof follows similar structure as in the analogous proof for the infinite-sample case. Here,
for all $s$, the outer loop updates for ANIL can be written as:
\begin{align}
\mathbf{w}_{s+1} &= \mathbf{w}_s - \frac{\beta}{n}\sum_{i=1}^n \nabla_{\mathbf{w}} \hat{\mathcal{L}}_i(\mathbf{{B}}_s, \mathbf{w}_{s,i},\mathcal{D}_i^{in}) = \mathbf{w}_{s} -  \frac{ \beta}{n}\sum_{i=1}^n \mathbf{B}_s^\top \mathbf{\Sigma}_{t,i}^{out}\mathbf{B}_s \mathbf{w}_{s,i} + \frac{\beta}{n}\sum_{i=1}^n \mathbf{{B}}_s^\top \mathbf{\Sigma}_{t,i}^{out}\mathbf{{B}}_\ast \mathbf{w}_{\ast,s,i} \nonumber \\
&= \mathbf{w}_{s} -  \frac{ \beta}{n}\sum_{i=1}^n \mathbf{B}_s^\top \mathbf{B}_s \mathbf{w}_{s,i} + \frac{\beta}{n}\sum_{i=1}^n \mathbf{{B}}_s^\top\mathbf{B}_\ast \mathbf{w}_{\ast,s,i} + \frac{ \beta}{n}\sum_{i=1}^n\mathbf{B}_s^\top (\mathbf{I}_d - \mathbf{\Sigma}_{s,i}^{out})(\mathbf{B}_s \mathbf{w}_{s,i} -\mathbf{B}_\ast \mathbf{w}_{\ast,s,i} )\nonumber \\ \label{upd_head_anil_out_pop}
\end{align}
% Assume for now that the columns of $\mathbf{B}_t$ are orthogonalized, i.e. $\mathbf{B}_t=\mathbf{\hat{B}}_t$ such that $\mathbf{\hat{B}}_t^\top \mathbf{\hat{B}}_t = \mathbf{I}_k$ (we should be able to later show that this assumption is WLOG). 
% We also have that $\mathbf{\hat{B}}_\ast$ is orthogonal, so we can also denote it by $ \mathbf{\hat{B}}_\ast$. 
Substituting the definition of $\mathbf{w}_{s,i} = \mathbf{w}_s  - \alpha \mathbf{B}_s^\top \mathbf{B}_s \mathbf{w}_s + \alpha \mathbf{B}_s^\top \mathbf{B}_{\ast} \mathbf{w}_{\ast,s,i} +\alpha \mathbf{B}_s^\top(\mathbf{I}_d - \mathbf{\Sigma}_{s,i}^{in})(\mathbf{B}_s \mathbf{w}_s - \mathbf{B}_\ast \mathbf{w}_{\ast,s,i})$, we have \begin{align}
\mathbf{w}_{s+1}
&= (\mathbf{I}_{k}\! - \! \beta (\mathbf{I}- \alpha\mathbf{B}_s^\top \mathbf{B}_s) \mathbf{B}_s^\top \mathbf{B}_s)\mathbf{w}_s +
\beta (\mathbf{I}- \alpha\mathbf{B}_s^\top \mathbf{B}_s)\mathbf{{B}}_s^\top \mathbf{{B}}_\ast \frac{1}{n}\sum_{i=1}^n\mathbf{w}_{\ast,s,i}  \nonumber \\
&\quad - \frac{\beta \alpha}{n}\sum_{i=1}^n \mathbf{B}_s^\top \mathbf{B}_s \mathbf{B}_s^\top(\mathbf{I}_d - \mathbf{\Sigma}_{t,i}^{in})(\mathbf{B}_s \mathbf{w}_s - \mathbf{B}_\ast \mathbf{w}_{\ast,s,i}) \nonumber \\
&\quad + \frac{ \beta}{n}\sum_{i=1}^n\mathbf{B}_s^\top (\mathbf{I}_d - \mathbf{\Sigma}_{t,i}^{out})(\mathbf{B}_s \mathbf{w}_{s,i} -\mathbf{B}_\ast \mathbf{w}_{\ast,s,i} ) 
\end{align}
{
% \color{blue}
In the exact ANIL case, we have
\begin{align}
    \mathbf{w}_{s+1}
&= (\mathbf{I}_{k}\! - \! \beta (\mathbf{I}- \alpha\mathbf{B}_s^\top \mathbf{B}_s) \mathbf{B}_s^\top \mathbf{B}_s(\mathbf{I}- \alpha\mathbf{B}_s^\top \mathbf{B}_s))\mathbf{w}_s +
\beta (\mathbf{I}- \alpha\mathbf{B}_s^\top \mathbf{B}_s)^2\mathbf{{B}}_s^\top \mathbf{{B}}_\ast \frac{1}{n}\sum_{i=1}^n\mathbf{w}_{\ast,s,i}  \nonumber \\
&\quad -(\mathbf{I}- \alpha\mathbf{B}_s^\top \mathbf{B}_s) \frac{\beta \alpha}{n}\sum_{i=1}^n \mathbf{B}_s^\top \mathbf{B}_s \mathbf{B}_s^\top(\mathbf{I}_d - \mathbf{\Sigma}_{t,i}^{in})(\mathbf{B}_s \mathbf{w}_s - \mathbf{B}_\ast \mathbf{w}_{\ast,s,i}) \nonumber \\
&\quad + (\mathbf{I}- \alpha\mathbf{B}_s^\top \mathbf{B}_s)\frac{ \beta}{n}\sum_{i=1}^n\mathbf{B}_s^\top (\mathbf{I}_d - \mathbf{\Sigma}_{t,i}^{out})(\mathbf{B}_s \mathbf{w}_{s,i} -\mathbf{B}_\ast \mathbf{w}_{\ast,s,i} )  \nonumber \\
&\quad + \frac{\beta \alpha}{n}\sum_{i=1}^n (\mathbf{B}_s^\top \mathbf{B}_s - \mathbf{B}_s^\top \mathbf{\Sigma}_{t,i}^{out} \mathbf{B}_s) \mathbf{B}_s^\top \mathbf{B}_s(\mathbf{I}- \alpha\mathbf{B}_s^\top \mathbf{B}_s)\mathbf{w}_s \nonumber \\
&\quad +
\frac{\beta \alpha }{n}\sum_{i=1}^n  (\mathbf{B}_s^\top \mathbf{B}_s - \mathbf{B}_s^\top \mathbf{\Sigma}_{t,i}^{out} \mathbf{B}_s)(\mathbf{I}- \alpha\mathbf{B}_s^\top \mathbf{B}_s)\mathbf{{B}}_s^\top \mathbf{{B}}_\ast \mathbf{w}_{\ast,s,i}  \nonumber \\
&\quad -\frac{\beta \alpha^2}{n}\sum_{i=1}^n (\mathbf{B}_s^\top \mathbf{B}_s - \mathbf{B}_s^\top \mathbf{\Sigma}_{t,i}^{out} \mathbf{B}_s)  \mathbf{B}_s^\top \mathbf{B}_s \mathbf{B}_s^\top(\mathbf{I}_d - \mathbf{\Sigma}_{t,i}^{in})(\mathbf{B}_s \mathbf{w}_s - \mathbf{B}_\ast \mathbf{w}_{\ast,s,i}) \nonumber \\
&\quad + \frac{ \beta \alpha}{n}\sum_{i=1}^n(\mathbf{B}_s^\top \mathbf{B}_s - \mathbf{B}_s^\top \mathbf{\Sigma}_{t,i}^{out} \mathbf{B}_s)\mathbf{B}_s^\top (\mathbf{I}_d - \mathbf{\Sigma}_{t,i}^{out})(\mathbf{B}_s \mathbf{w}_{s,i} -\mathbf{B}_\ast \mathbf{w}_{\ast,s,i} )  \nonumber 
\end{align}
}
% {\color{red}
% Issue with using same data to compute Hessian as for the rest of the outer loop update: we get 4th order moments, which introduce a bias term, so the population case analysis isn't quite correct. For Gaussian data, we can compute the bias explicitly. For generic sub-gaussian we cannot.
% \begin{align}
%     &\mathbb{E}[\frac{ \beta \alpha}{n}\sum_{i=1}^n\mathbf{B}_s^\top \mathbf{\Sigma}_{t,i}^{out} \mathbf{B}_s\mathbf{B}_s^\top \mathbf{\Sigma}_{t,i}^{out}(\mathbf{B}_s \mathbf{w}_{s,i} -\mathbf{B}_\ast \mathbf{w}_{\ast,s,i} ) ] \nonumber \\
%     &\neq \frac{ \beta \alpha}{n}\sum_{i=1}^n\mathbf{B}_s^\top  \mathbf{B}_s\mathbf{B}_s^\top(\mathbf{B}_s \mathbf{w}_{s,i} -\mathbf{B}_\ast \mathbf{w}_{\ast,s,i} )  \nonumber
% \end{align}
% Empirically, noise ceiling is $\approx 0.5$. If $\mathbf{w}_0$ has norm 1, then it decreases in the long run (may increase to start) and we still have linear convergence.

% Either we can assume that different data is used for hessian approximation, or assume gaussian data (but then we need to change population analysis)

% With different data for hessian, 
% }

Let $a_s \coloneqq \|\mathbf{w}_s\|_2$ for all $s\in\{0,\dots,t\!+\!1\}$. Note that $\bigcup_{s=0}^t A_3(s)$ implies $\sigma_{\max}(\mathbf{B}_s^\top \mathbf{B}_s) \leq \frac{1+\tau}{\alpha}< \frac{2}{\alpha}$ for all $s\in\{0,\dots,t\!+\!1\}$. Also, we have shown 
\begin{align}
   \left\| \frac{\beta \alpha}{n}\sum_{i=1}^n \mathbf{B}_s^\top \mathbf{B}_s \mathbf{B}_s^\top(\mathbf{I}_d - \mathbf{\Sigma}_{s,i}^{in})(\mathbf{B}_s \mathbf{w}_s - \mathbf{B}_\ast \mathbf{w}_{\ast,s,i}) \right\|_2 &\leq \tfrac{\beta}{\alpha}\delta_{in}a_s + \tfrac{\beta}{\sqrt{\alpha}}\delta_{in} L_\ast \nonumber \\
  \left\|\frac{ \beta}{n}\sum_{i=1}^n\mathbf{B}_s^\top (\mathbf{I}_d - \mathbf{\Sigma}_{s,i}^{out})(\mathbf{B}_s \mathbf{w}_{s,i} -\mathbf{B}_\ast \mathbf{w}_{\ast,s,i} ) \right\|_2 &\leq \frac{\beta}{\alpha}\delta_{out}\|\mathbf{w}_{s,i}\|_2 +\frac{\beta}{\sqrt{\alpha}}\delta_{out}L_\ast \nonumber \\
  &\leq \frac{\beta}{\alpha}\delta_{out}(\|\mathbf{I}_k\!-\!\alpha \mathbf{B}_s^\top \mathbf{B}_s\|_2 a_s\!+\!\sqrt{\alpha} L_\ast + \delta_{in}a_s\!+\!\sqrt{\alpha} \delta_{in} L_\ast)\nonumber \\ &\quad \!+\!\frac{\beta}{\sqrt{\alpha}}\delta_{out}L_\ast \nonumber \\
  &\leq  \frac{\beta}{\alpha}\delta_{out}(\|\mathbf{I}_k - \alpha \mathbf{B}_s^\top \mathbf{B}_s\|_2 a_s + \sqrt{\alpha} L_\ast + \delta_{in}a_s) +\frac{\beta}{\sqrt{\alpha}}\delta_{out}L_\ast \nonumber 
\end{align}
with high probability.

{\color{blue} For Exact ANIL, we have 
\begin{align}
    a_{s+1} &\leq a_s + \frac{\beta}{\sqrt{\alpha}}\tau_s^2 \eta_\ast + \frac{\beta}{{\alpha}}\tau_s(\delta_{in}+\delta_{out}(\tau_s +  \delta_{in})a_s + \frac{\beta}{\sqrt{\alpha}}\tau_s\delta_{out}(\dist_s + \tau_s  +\sqrt{\alpha}\delta_{in})  L_\ast  \nonumber \\
    &\quad + \frac{\beta}{\alpha}\tau_s \delta_{H}(a_s + \sqrt{\alpha} L_\ast)+ \frac{\beta }{\alpha}\delta_{H} \delta_{in} (a_s+\sqrt{\alpha} L_\ast) + \frac{\beta}{\alpha} \delta_{H}(\tau_s a_s +\delta_{in} a_s +\dist_s L_\ast + \tau_s L_\ast + \sqrt{\alpha}\delta_{in}L_\ast) \nonumber 
\end{align}
% why do stochastic processes with mean zero noise not diverge? besides azuma hoeffding
% we have terms with no $a_s$ and no $\tau_s$, and these terms are not summable

}

% Using this fact with \eqref{uuu}, we obtain
% \begin{align}
%     a_{s+1} &\leq \left(1 + (2+\delta_{out})\tfrac{\beta}{\alpha} \|\mathbf{I}_k - \alpha \mathbf{B}_s^\top \mathbf{B}_s\|_2 + \frac{\beta}{\alpha}\delta_{in}\right)a_s + \tfrac{2\beta}{\sqrt{\alpha}} \|\mathbf{I}_k - \alpha \mathbf{B}_s^\top \mathbf{B}_s\|_2 L_\ast \nonumber \\
%     &\quad + \frac{\beta}{\sqrt{\alpha}} (\delta_{in}+\delta_{out}) L_\ast
%     \label{foralll}
%     %\nonumber \\
%     % &\leq a_0\prod_{s=1}^t(1+\tfrac{\beta}{\alpha}{z}_s) +\tfrac{\beta}{\sqrt{\alpha}} L_\ast \sum_{s=1}^t {z}_s\prod_{r=s+1}^t(1+ \tfrac{\beta}{\alpha}z_r) \nonumber \\
%     % &=  \tfrac{\beta}{\sqrt{\alpha}} L_\ast \sum_{s=1}^t z_s\prod_{r=s+1}^t(1+ \tfrac{\beta}{\alpha}z_r) \nonumber \\
%     % &= \tfrac{\beta}{\sqrt{\alpha}} L_\ast \sum_{s=1}^t \rho^{s} \tfrac{\alpha^{2}\beta^2 L_\ast^4 }{1- \rho}\prod_{r=s+1}^t(1+ \rho^{r} \tfrac{{\alpha}\beta^3L_\ast^4 }{1- \rho}) \nonumber \\
%     % &= \tfrac{\alpha^{1.5}\beta^3 L_\ast^4 }{1 - \rho} L_\ast \sum_{s=0}^t \rho^{s} \prod_{r=s+1}^t\left(1+ \rho^{r} \tfrac{{\alpha}\beta^3L_\ast^4 }{1 - \rho}\right) \nonumber
% \end{align}  
% {\color{blue} In the exact ANIL case, we have 
% \begin{align}
%     a_{s+1} &\leq (1+)
% \end{align}
% }
% {\color{red} We have problems because the $\delta$'s are not summable....}

% for all $s\in\{0,\dots,t\!+\!1\}$.

\end{proof}
