# Supplementary material for: MAML and ANIL Provably Learn Representations
Source: arXiv:2202.03483 source file (2023-06-04)
Supplement: Supplementary file 2 [file Appendix_MAML_new_FS.tex]

\newpage
\subsection{Finite Samples}

Now we consider the case of general $m_{in}$ and $m_{out}$. Proof outline:

Use earlier lemma bounding closeness of wti to pop wti

New lemma bounding closeness of Bti to pop Bti

Outer loop update: split into 3 terms: 1) pop plus inner loop errors 2) outer loop errors minus noise plus inner loop errors 3) outer loop noise errors plus inner loop errors.

We start by showing the concentration of each $\mathbf{B}_{t,i}$ to the infinite-sample update. We have
\begin{align}
    \mathbf{B}_{t,i} &= \mathbf{B}_{t,i,pop} + \mathbf{S}_{t,i,in} \nonumber \\
    \mathbf{S}_{t,i,in}&\coloneqq -\alpha \left(\mathbf{I}_d - \mathbf{\Sigma}_{i,in}\right)(\mathbf{B}_t \mathbf{w}_t \mathbf{w}_t^\top  - \mathbf{B}_\ast \mathbf{w}_{\ast,i} \mathbf{w}_t^\top ) + \frac{\alpha}{m_{in}}\mathbf{X}_{i,in}\mathbf{z}_{i,in}\mathbf{w}_{t}^\top
\end{align}

\begin{lemma}
We have $\mathbf{S}^{in}_{t,i} = $ 
\end{lemma}

\begin{proof}

\end{proof}

The outer loop update for the representation is:
\begin{align}
    \mathbf{B}_{t+1} &= \mathbf{B}_{t+1,pop,+} + \mathbf{S}_{t+1,out} \nonumber \\
    \mathbf{S}_{t+1,out}&\coloneqq 
    % -\beta\frac{1}{n}\sum_{i=1}^n \left(\mathbf{I}_d - \mathbf{\Sigma}_{i,out}\right)(\mathbf{B}_{t,i} \mathbf{w}_{t,i} \mathbf{w}_{t,i}^\top  - \mathbf{B}_\ast \mathbf{w}_{\ast,i} \mathbf{w}_{t,i}^\top ) +\beta \frac{1}{nm_{out}}\sum_{i=1}^n\mathbf{X}_{i,out}\mathbf{z}_{i,out}\mathbf{w}_{t,i}^\top \nonumber \\
    % &= 
    -\beta\frac{1}{n}\sum_{i=1}^n \left( \mathbf{\Sigma}_{i,out} - \mathbf{I}_d \right)(\mathbf{B}_{t,i,pop} \mathbf{w}_{t,i} \mathbf{w}_{t,i}^\top  - \mathbf{B}_\ast \mathbf{w}_{\ast,i} \mathbf{w}_{t,i}^\top ) +\beta \frac{1}{nm_{out}}\sum_{i=1}^n\mathbf{X}_{i,out}\mathbf{z}_{i,out}\mathbf{w}_{t,i}^\top \nonumber \\
    &\quad  -\beta\frac{1}{n}\sum_{i=1}^n  \mathbf{\Sigma}_{i,out} \mathbf{S}_{t,i,in} \mathbf{w}_{t,i} \mathbf{w}_{t,i}^\top \nonumber \\
    % - \mathbf{B}_\ast \mathbf{w}_{\ast,i} \mathbf{w}_{t,i}^\top )\nonumber \\
    % &\quad -\beta\frac{1}{n}\sum_{i=1}^n \left(\mathbf{I}_d - \mathbf{\Sigma}_{i,out}\right)(\mathbf{S}_{t,i,in} \mathbf{w}_{t,i} \mathbf{w}_{t,i}^\top) \nonumber \\
    % \mathbf{B}_{t+1,pop}' &= \mathbf{B}_{t+1,pop,+} +\mathbf{S}_{t+1,out}' \nonumber \\
    % \mathbf{S}_{t,i,out}' &= 
    % % -\beta \frac{1}{n}\sum_{i=1}^n \mathbf{S}_{t,i,in}\mathbf{w}_{t,i}\mathbf{w}_{t,i}^\top
    % - \beta \lambda \alpha \frac{1}{n}\sum_{i=1}^n \mathbf{S}_{t,i,in}(\alpha \mathbf{B}_{t,i}^\top \mathbf{B}_{t,i} - \mathbf{I}_k)
\end{align}
so we need to bound
\begin{align}
&\|\mathbf{B}_{\ast,\perp}^\top\mathbf{B}_{t+1}\|_2\nonumber \\    &=\|\mathbf{B}_{\ast,\perp}^\top(\mathbf{B}'_{t+1,pop}+
    \mathbf{S}_{t+1,out})\|_2 \nonumber\\
    &= \|\mathbf{B}_{\ast,\perp}^\top(\mathbf{B}_{t+1,pop,+}+ \mathbf{S}'_{t+1,out}+
    \mathbf{S}_{t+1,out})\|_2 \nonumber\\
    &\leq \|\mathbf{B}_{\ast,\perp}^\top\mathbf{B}_{t+1,pop,+}\|_2 + \|\mathbf{B}_{\ast,\perp}^\top(\mathbf{S}'_{t+1,out}+
    \mathbf{S}_{t+1,out})\|_2 \nonumber\\
    &\leq {\color{blue}\|\mathbf{B}_{\ast,\perp}^\top \mathbf{B}_{t+1,pop,+}\|_2 }\nonumber \\
    &\quad + {\color{blue}\left\|\mathbf{B}_{\ast,\perp}^\top\left(\beta\frac{1}{n}\sum_{i=1}^n \left( \mathbf{\Sigma}_{i,out}-\mathbf{I}_d \right)(\mathbf{B}_{t,i,pop} \mathbf{w}_{t,i} \mathbf{w}_{t,i}^\top  - \mathbf{B}_\ast \mathbf{w}_{\ast,i} \mathbf{w}_{t,i}^\top )  \right) \right\|_2} \nonumber \\
    &\quad + {\color{blue}\left\|\mathbf{B}_{\ast,\perp}^\top\left( \beta \frac{1}{nm_{out}}\sum_{i=1}^n\mathbf{X}_{i,out}\mathbf{z}_{i,out}\mathbf{w}_{t,i}^\top \right) \right\|_2} \nonumber \\
    &\quad + {\color{red}\left\|\mathbf{B}_{\ast,\perp}^\top\left(\beta\frac{1}{n}\sum_{i=1}^n ( \mathbf{\Sigma}_{i,out} - \mathbf{I}_d)\mathbf{S}_{t,i,in} \mathbf{w}_{t,i} \mathbf{w}_{t,i}^\top\right) \right\|_2} \nonumber \\
    &\quad + {\color{red}\left\|\mathbf{B}_{\ast,\perp}^\top\left(\beta\frac{1}{n}\sum_{i=1}^n \mathbf{S}_{t,i,in} \mathbf{w}_{t,i} \mathbf{w}_{t,i}^\top\right) \right\|_2}
\end{align}
% For last term, use $P(ab \leq c) \geq P(a \leq \sqrt{c} \text{ and } b \leq \sqrt{c})=  1 - P(a > \sqrt{c} \text{ or } b > \sqrt{c}) \geq 1 - P(a > \sqrt{c}) - P(b > \sqrt{c})$. Will get sth like $(1+\delta_{out})(\delta_{in}...)$

% empirically: inner loop samples can be bounded by taking the max. outer loop samples must be bounded by averaging over n. the challenge remains to bound the max of the inner loop samples. We have 6th order products of sub-gaussians. need to show that these go zero. dimension dependence - we should still have a rt(d) dependence in the inner loop bound, but empirically this doesn't seem to matter...

% strangely, max over the in still works even with large d. this implies that true neighborhood size is like 

two questions: 1) does bound on term with only in grow with d. if it does, then we can bound it. if it doesn't, then we need to regroup the terms
2) 

3) is bound for ANIL correct (does error really not go to 0 as min goes to infinity)? if wrong, fix may have to do with showing that tau is going to zero. but this isn't true in FS sample case?

need to get bound that is like:

$\frac{dk}{n m_{in}} + \frac{dk}{n m_{out}}$

why is 3rd term so large??

first term grows with d, as expected, but it is not dominant... what is dominant? third term? but why is it so big?

we know the neighborhood size is increasing with d/(n min) (note discrepancy with anil)... let's just bound it as such. need concentration of 3x covariance matrices.

% what can we do to improve bound on $\|\mathbf{w}_t\|_2\leq \|\mathbf{w}_{t-1}\|_2$ 

Note that the $\mathbf{w}_{t,i}$'s also have noise but we have already controlled them earlier.

First step: bound $(\alpha \mathbf{B}_{t,i}^\top \mathbf{B}_{t,i} - \mathbf{I}_k)$.
We have 
\begin{align}
    \alpha \mathbf{B}_{t,i}^\top \mathbf{B}_{t,i} - \mathbf{I}_k &= \alpha \mathbf{B}_{t,i,pop}^\top \mathbf{B}_{t,i,pop} - \mathbf{I}_k + \alpha  \mathbf{S}_{t,i,in}^\top \mathbf{B}_{t,i,pop}+ \alpha \mathbf{B}_{t,i,pop}^\top  \mathbf{S}_{t,i,in} + \alpha \mathbf{S}_{t,i,in}^\top \mathbf{S}_{t,i,in}
\end{align}
Empirically, this is bounded by something that grows with $d$. So we need to

For FO-MAML:
\begin{align}
    \nabla_{\mathbf{B}} \hat{F}_{t,i}(\mathbf{B}_t, \w)&=  \nonumber \\
    \nabla_{\w}\hat{F}_{t,i}(\b,\w) &=   \nonumber
\end{align}

\begin{align}
        \mathbf{B}_{t+1} &= \mathbf{B}_{t+1,pop,+} + \mathbf{S}_{t+1,out} \nonumber \\
    \mathbf{S}_{t+1,out}&\coloneqq 
    -\beta\frac{1}{n}\sum_{i=1}^n \left( \mathbf{\Sigma}_{i,out} - \mathbf{I}_d \right)(\mathbf{B}_{t,i,pop} \mathbf{w}_{t,i} \mathbf{w}_{t,i}^\top  - \mathbf{B}_\ast \mathbf{w}_{\ast,i} \mathbf{w}_{t,i}^\top ) +\beta \frac{1}{nm_{out}}\sum_{i=1}^n\mathbf{X}_{i,out}\mathbf{z}_{i,out}\mathbf{w}_{t,i}^\top \nonumber \\
    &\quad  -\beta\frac{1}{n}\sum_{i=1}^n  \mathbf{\Sigma}_{i,out} \mathbf{S}_{t,i,in} \mathbf{w}_{t,i} \mathbf{w}_{t,i}^\top \nonumber
\end{align}
First terms: to get rid of outer loop samples, the first terms are easy, one d and two ks. 

but to control B wwT 

we can again use the same trick?

issue is that we can't control the mean. also, we have terms with double products, plus the terms with triple products... finish ANIL analysis then do MAML. Maybe can use separate samples for B and w for MAML. This would make things much easier.

and third terms are difficult to control.
