# Supplementary material for: MAML and ANIL Provably Learn Representations
Source: arXiv:2202.03483 source file (2023-06-04)
Supplement: Supplementary file 3 [file old_Appendix_ANIL_FS.tex]

\section{Finite Samples}
% We start by abstracting 

% {\em Note: I removed the old Lemma 1 - Liam}

\begin{align}
    \mathbf{w}_{t,i} %&= \mathbf{w}_t - \alpha \mathbf{\hat{B}}_t^\top \sum_{j=1}^{m_{in}}\mathbf{x}_{i,j}\mathbf{x}_{i,j}^\top \mathbf{\hat{B}}_t \mathbf{{w}}_t  + \alpha \mathbf{\hat{B}}_t^\top \frac{1}{m_{in}}\sum_{j=1}^{m_{in}}\mathbf{x}_{i,j}\mathbf{x}_{i,j}^\top \mathbf{\hat{B}}_\ast \mathbf{{w}}_{\ast,i} \nonumber \\
    &= \mathbf{w}_t - \alpha \nabla_{\mathbf{w}} \hat{f}_i(\mathbf{B}_t, \mathbf{w}_t, \mathcal{D}_{i}^{in}) =  (\mathbf{I}_k- \alpha\mathbf{\hat{B}}_t^\top \mathbf{\Sigma}_{i}^{in} \mathbf{\hat{B}}_t)\mathbf{{w}}_t + \alpha \mathbf{\hat{B}}_t^\top \mathbf{\Sigma}_{i}^{in} \mathbf{\hat{B}}_\ast\mathbf{{w}}_{\ast,i} + \frac{\alpha}{m_{in}} \mathbf{\hat{B}}_t^\top \mathbf{X}_{i}^{in}\mathbf{z}_{i}^{in}. \label{upd_head_anil}
\end{align}
The outer loop updates for the head and representation are:
\begin{align}
\mathbf{w}_{t+1} &= \mathbf{w}_t - \frac{\beta}{n}\sum_{i=1}^n \nabla_{\mathbf{w}} \hat{f}_i(\mathbf{\hat{B}}_t, \mathbf{w}_{t,i}) \\
&= \label{upd_head_out_anil} \\
    \mathbf{{B}}_{t+1} &= \mathbf{\hat{B}}_t  - \frac{\beta}{nm_{out}}\sum_{i=1}^n\sum_{j=1}^{m_{out}} \mathbf{x}_{i,j}\mathbf{x}_{i,j}^\top \mathbf{\hat{B}}_t  \mathbf{w}_{t,i}\mathbf{w}_{t,i}^\top + \frac{\beta}{n m_{out}} \sum_{i=1}^n \sum_{j=1}^{m_{out}} \mathbf{x}_{i,j}\mathbf{x}_{i,j}^\top \mathbf{\hat{B}}_\ast\mathbf{w}_{\ast,i} \mathbf{w}_{t,i}^\top  \label{upd_rep_anil} \\
    \mathbf{\hat{B}}_{t+1}, \mathbf{R}_{t+1} &= \text{QR}(\mathbf{\bar{B}}_{t+1})
\end{align}


The update for $\mathbf{B}$ is:
\begin{align}
    \mathbf{B}_{t+1} &= \mathbf{\hat{B}}_t  - \frac{\beta}{nm_{out}}\sum_{i=1}^n\sum_{j=1}^{m_{out}} \mathbf{x}_{i,j}\mathbf{x}_{i,j}^\top \mathbf{\hat{B}}_t  \mathbf{w}_{t,i}\mathbf{w}_{t,i}^\top + \frac{\beta}{n m_{out}} \sum_{i=1}^n \sum_{j=1}^{m_{out}} \mathbf{x}_{i,j}\mathbf{x}_{i,j}^\top \mathbf{\hat{B}}_\ast\mathbf{w}_{\ast,i} \mathbf{w}_{t,i}^\top  \nonumber \\
    &= \mathbf{\hat{B}}_t\left(\mathbf{I} - \frac{\beta}{n}\sum_{i=1}^n \mathbf{w}_{t,i}\mathbf{w}_{t,i}^\top\right) + \mathbf{\hat{B}}_\ast\left(\frac{\beta}{n} \sum_{i=1}^n \mathbf{w}_{\ast,i} \mathbf{w}_{t,i}^\top \right) \nonumber \\
    &\quad + \frac{\beta}{n} \sum_{i=1}^n \left(\mathbf{I}_d - \frac{1}{m_{out}}\sum_{j=1}^{m_{out}} \mathbf{x}_{i,j}\mathbf{x}_{i,j}^\top \right) \mathbf{\hat{B}}_t  \mathbf{w}_{t,i}\mathbf{w}_{t,i}^\top  - \frac{\beta}{n} \sum_{i=1}^n \left(\mathbf{I}_d - \frac{1}{m_{out}}\sum_{j=1}^{m_{out}} \mathbf{x}_{i,j}\mathbf{x}_{i,j}^\top \right) \mathbf{\hat{B}}_\ast \mathbf{w}_{\ast,i}\mathbf{w}_{t,i}^\top  
\end{align}


\begin{assumption}
The ground-truth heads satisfy the following two properties:
\begin{enumerate} \label{assump:gt}
    \item (Task normalization) For all $i\in [n]$, $\|\mathbf{w}_{\ast,i}\|_2 \leq L_{\max}$. 
    % Note that this immediately implies
    \item (Task diversity) $
     0 \leq \mu_\ast^2 \leq  \sigma_{\min}\left(\frac{1}{n} \sum_{i=1}^n \mathbf{w}_{\ast,i}\mathbf{w}_{\ast,i}^\top \right) \leq
     \sigma_{\min}\left(\frac{1}{n} \sum_{i=1}^n \mathbf{w}_{\ast,i}\mathbf{w}_{\ast,i}^\top \right) \leq L_\ast^2 
 $. 
% $\sigma_{\max}\left(\frac{1}{n} \sum_{i=1}^n \mathbf{w}_{\ast,i}\mathbf{w}_{\ast,i}^\top \right) \leq .$
\end{enumerate}
\end{assumption}
Note that if the ground-truth heads are well-conditioned, then $\mu_{\ast}^2$ and $L_{\ast}^2$ will be close to $1/k$. Also, we always have $L_{\ast}^2\leq L_{\max}^2$.

\begin{assumption} \label{assump:wt}
The current iterate $\mathbf{w}_t$ satisfies $\|\mathbf{w}_t\|_2 \leq L_\max$.
\end{assumption}

\begin{assumption}
\label{assump:data}
For all $i,j$, the sample $\mathbf{x}_{i,j} \in \mathbb{R}^d$ is $\mathbf{I}_d$-sub-Gaussian, in the sense that $\mathbb{E}[\exp(\mathbf{v}^\top \mathbf{x}_{i,j})] \leq \exp \left(\frac{\|\mathbf{v}\|_2^2}{2}\right)$ for all $\mathbf{v}\in \mathbb{R}^d$.
\end{assumption}

\textbf{Notations}

\begin{itemize}
    \item $\mathbf{e}_i \coloneqq \mathbf{w}_{t,i} - \mathbf{\hat{B}}_t^\top \mathbf{\hat{B}}_\ast \mathbf{w}_{\ast,i}$
    \item $\mathbf{E} \coloneqq \begin{bmatrix}\vdots \\
    \mathbf{e}_i^\top \\
    \vdots
    \end{bmatrix}$ 
    % \item $\mathbf{W}_{t,in} \coloneqq \begin{bmatrix}\vdots \\
    % \mathbf{w}_{t,i}^\top \\
    % \vdots
    % \end{bmatrix} = ((\mathbf{I}_k - \mathbf{\hat{B}}_t^\top \mathbf{\Sigma}_{i,in} \mathbf{\hat{B}}_t)\mathbf{w}_t \mathbf{1}_n^\top + \mathbf{\hat{B}}_t^\top \mathbf{\Sigma}_{i,in} \mathbf{\hat{B}}_\ast \mathbf{W}_{\ast}^\top )^\top$
    \item $m_{in}$: number of inner loop samples. $m_{out}$: number of outer loop samples.
    \item $\mathbf{\Sigma}_{i,in} \coloneqq \frac{1}{m_{in}}\sum_{j=1}^{m_{in}}\mathbf{x}_{i,j}\mathbf{x}_{i,j}^\top$, $\mathbf{\Sigma}_{i,out} \coloneqq \frac{1}{m_{out}}\sum_{j=1}^{m_{out}}\mathbf{x}_{i,j}\mathbf{x}_{i,j}^\top$
\end{itemize}

\subsection{Finite inner loop samples}

\begin{lemma} \label{lem:concen}
Let $\alpha=1$. Under assumptions \ref{assump:gt}, \ref{assump:wt}, and \ref{assump:data}, we have 
\begin{align}
   \frac{1}{\sqrt{n}} \| \mathbf{E} \|_F \leq O\left(L_{\max} \frac{\sqrt{k}+ \sqrt{\log(n)}}{\sqrt{m_{in}}}\right)
\end{align}
with probability at least $1 - 4 n^{-99}$.
\end{lemma}
\begin{proof}
For some $i$, we have
\begin{align}
    \mathbf{w}_{t,i} &= \mathbf{w}_t - \alpha \mathbf{\hat{B}}_t^\top \sum_{j=1}^{m_{in}}\mathbf{x}_{i,j}\mathbf{x}_{i,j}^\top \mathbf{\hat{B}}_t \mathbf{{w}}_t  + \alpha \mathbf{\hat{B}}_t^\top \frac{1}{m_{in}}\sum_{j=1}^{m_{in}}\mathbf{x}_{i,j}\mathbf{x}_{i,j}^\top \mathbf{\hat{B}}_\ast \mathbf{{w}}_{\ast,i} \nonumber \\
    &= (\mathbf{I}- \alpha\mathbf{\hat{B}}_t^\top \mathbf{\Sigma}_{i,in} \mathbf{\hat{B}}_t)\mathbf{{w}}_t + \alpha \mathbf{\hat{B}}_t^\top \mathbf{\Sigma}_{i,in} \mathbf{\hat{B}}_\ast\mathbf{{w}}_{\ast,i}.
\end{align}
Thus, for $\alpha=1$,
\begin{align}
    \| \mathbf{w}_{t,i} - \mathbf{\hat{B}}_{t}^\top\mathbf{\hat{B}}_\ast{\mathbf{w}_{\ast,i}}\|_2 & = \|(\mathbf{I}- \mathbf{\hat{B}}_t^\top \mathbf{\Sigma}_{i,in} \mathbf{\hat{B}}_t)\mathbf{{w}}_t +  \mathbf{\hat{B}}_t^\top \mathbf{\Sigma}_{i,in} \mathbf{\hat{B}}_\ast\mathbf{{w}}_{\ast,i} - \mathbf{\hat{B}}_{t}^\top\mathbf{\hat{B}}_\ast{\mathbf{w}_{\ast,i}}\|_2\nonumber \\
    &\leq \|(\mathbf{I}- \mathbf{\hat{B}}_t^\top \mathbf{\Sigma}_{i,in} \mathbf{\hat{B}}_t)\mathbf{{w}}_t\|_2 + \| \mathbf{\hat{B}}_t^\top \mathbf{\Sigma}_{i,in} \mathbf{\hat{B}}_\ast\mathbf{{w}}_{\ast,i} - \mathbf{\hat{B}}_{t}^\top\mathbf{\hat{B}}_\ast{\mathbf{w}_{\ast,i}}\|_2 \nonumber \\
    &\leq  \|\mathbf{I}_k- \mathbf{\hat{B}}_t^\top \mathbf{\Sigma}_{i,in} \mathbf{\hat{B}}_t\|_2 \|  \mathbf{{w}}_t\|_2 + \| \mathbf{\hat{B}}_{t}^\top \mathbf{\Sigma}_{i,in} \mathbf{\hat{B}}_\ast - \mathbf{\hat{B}}_{t}^\top\mathbf{\hat{B}}_\ast\|_2 \|{\mathbf{w}_{\ast,i}}\|_2  \nonumber \\
    &\leq  L_{\max}\|\mathbf{I}_k- \mathbf{\hat{B}}_t^\top \mathbf{\Sigma}_{i,in} \mathbf{\hat{B}}_t\|_2  + L_{\max}\| \mathbf{\hat{B}}_{t}^\top \mathbf{\Sigma}_{i,in} \mathbf{\hat{B}}_\ast - \mathbf{\hat{B}}_{t}^\top\mathbf{\hat{B}}_\ast\|_2\label{twoterms}
\end{align}
where we have used $\|{\mathbf{w}_{\ast,i}}\|_2 \leq L_{\max}$ and $\|{\mathbf{w}_{t}}\|_2 \leq L_{\max}$. 
% (assumed for simplicity, but we can likely show that we can normalize $\mathbf{w}_t$ at the end of each round WLOG). 
We first consider the term 
\begin{align}
    \|\mathbf{I}_k- \mathbf{\hat{B}}_t^\top \mathbf{\Sigma}_{i,in} \mathbf{\hat{B}}_t\|_2  &=  \left\|\mathbf{I}_k-    \frac{1}{m_{in}}\sum_{j=1}^{m_{in}}\mathbf{\hat{B}}_t^\top\mathbf{x}_{i,j}\mathbf{x}_{i,j}^\top\mathbf{\hat{B}}_t\right\|_2
\end{align}
where $\mathbf{\hat{B}}_t^\top\mathbf{x}_{i,j}$ is sub-Gaussian with covariance $\mathbf{\hat{B}}_t^\top\mathbf{\hat{B}}_t = \mathbf{I}_k$. Thus, by equation 4.22 in Vershynin, we have
\begin{align}
    \|\mathbf{I}_k- \mathbf{\hat{B}}_t^\top \mathbf{\Sigma}_{i,in} \mathbf{\hat{B}}_t\|_2 &\leq c  \max\left( \frac{\sqrt{k} + \lambda}{\sqrt{m_{in}}},  \frac{k + \lambda^2}{m_{in}}\right) \label{concen1}
\end{align}
for some absolute constant $c$,
with probability at least $ 1 - 2 e^{-\delta^2}$, for any $\lambda > 0$. The same bound holds for the second term in \eqref{twoterms}, so via a union bound we have 
\begin{align}
    \| \mathbf{w}_{t,i} - \mathbf{\hat{B}}_{t}^\top\mathbf{\hat{B}}_\ast{\mathbf{w}_{\ast,i}}\|_2 &\leq c' L_{\max} \max\left( \frac{\sqrt{k} + \lambda}{\sqrt{m_{in}}},  \frac{k + \lambda^2}{m_{in}}\right)
\end{align}
with probability at least $ 1 - 4 e^{-\lambda^2}$, for any $\lambda>0$. Now choose $\lambda = 10 \sqrt{\log(n)}$ and union bound over all $i \in [n]$ to obtain
\begin{align}
    \frac{1}{n}\sum_{i=1}^n\| \mathbf{w}_{t,i} - \mathbf{\hat{B}}_{t}^\top\mathbf{\hat{B}}_\ast{\mathbf{w}_{\ast,i}}\|_2^2 &\leq c'' L_{\max}^2  \left(\max\left( \frac{\sqrt{k} + 10 \sqrt{\log(n)}}{\sqrt{m_{in}}},  \frac{k + 100\log(n)}{m_{in}}\right)\right)^2 \nonumber \\
    \implies \frac{1}{\sqrt{n}}\|\mathbf{E}\|_F \leq \sqrt{\frac{1}{n}\sum_{i=1}^n\| \mathbf{w}_{t,i} - \mathbf{\hat{B}}_{t}^\top\mathbf{\hat{B}}_\ast{\mathbf{w}_{\ast,i}}\|_2^2} &\leq c' L_{\max} \max\left( \frac{\sqrt{k} + 10 \sqrt{\log(n)}}{\sqrt{m_{in}}},  \frac{k + 100\log(n)}{m_{in}}\right) %=: L_\ast \epsilon
\end{align}
with probability at least $1 - 4n^{-99}$. 
\end{proof}



\begin{lemma} \label{lem:cond}
Let $\beta = O(1/L_{\ast}^2)$.
Define $\mu^2 \coloneqq \sigma_{\min}\left(\frac{1}{n} \sum_{i=1}^n \mathbf{w}_{t,i}\mathbf{w}_{t,i}^\top \right)$, $L^2 \coloneqq \sigma_{\max}\left(\frac{1}{n} \sum_{i=1}^n \mathbf{w}_{t,i}\mathbf{w}_{t,i}^\top \right)$, and $\delta_{in} \coloneqq c\frac{\sqrt{k}+ 10 \sqrt{\log(n)}}{\sqrt{m_{in}}}$ for some absolute constant $c$. 
Under Assumptions \ref{assump:gt}, \ref{assump:wt} and \ref{assump:data}, we have 
\begin{align}
    L^2 &\leq L_{\max}^2 (2\delta_{in}+1)^2  \nonumber \\
    \text{and} \quad \mu^2 &\geq \mu_\ast^2 E_0 - 4 L_{\max}^2 (\delta_{in} + \delta_{in}^2) 
 \end{align}
 with probability at least $1 - 4 n^{-99}$.
\end{lemma}

\begin{proof}
Note that
\begin{align}
   \left\| \frac{1}{n} \sum_{i = 1}^n \mathbf{w}_{t,i}\mathbf{w}_{t,i}^\top\right\|_2 &= %\left\| \frac{1}{n}  \mathbf{W}_{t,in}^\top \mathbf{W}_{t,in}\right\|_2 \nonumber \\&= %\frac{1}{n}\left\|\mathbf{W}_{t,in}\right\|_2^2 \nonumber \\&= 
   \frac{1}{n}\Big\|\sum_{i=1}^n (\mathbf{I}_k - \mathbf{\hat{B}}_t^\top \mathbf{\Sigma}_{i,in} \mathbf{\hat{B}}_t)\mathbf{w}_t\mathbf{w}_t^\top (\mathbf{I}_k - \mathbf{\hat{B}}_t^\top \mathbf{\Sigma}_{i,in} \mathbf{\hat{B}}_t)  + \mathbf{\hat{B}}_t^\top \mathbf{\Sigma}_{i,in} \mathbf{\hat{B}}_\ast \mathbf{w}_{\ast,i} \mathbf{w}_{\ast,i}^\top  \mathbf{\hat{B}}_t \mathbf{\Sigma}_{i,in} \mathbf{\hat{B}}_\ast^\top  \nonumber \\
   &\quad + (\mathbf{I}_k - \mathbf{\hat{B}}_t^\top \mathbf{\Sigma}_{i,in} \mathbf{\hat{B}}_t)\mathbf{w}_t\mathbf{w}_{\ast,i}^\top  \mathbf{\hat{B}}_t \mathbf{\Sigma}_{i,in} \mathbf{\hat{B}}_\ast^\top + 
   \mathbf{\hat{B}}_t^\top \mathbf{\Sigma}_{i,in} \mathbf{\hat{B}}_\ast \mathbf{w}_{\ast,i}
   \mathbf{w}_t^\top (\mathbf{I}_k - \mathbf{\hat{B}}_t^\top \mathbf{\Sigma}_{i,in} \mathbf{\hat{B}}_t) 
   \Big\|_2^2 \nonumber \\
   &\leq \frac{1}{n}\Big\|\sum_{i=1}^n (\mathbf{I}_k - \mathbf{\hat{B}}_t^\top \mathbf{\Sigma}_{i,in} \mathbf{\hat{B}}_t)\mathbf{w}_t\mathbf{w}_t^\top (\mathbf{I}_k - \mathbf{\hat{B}}_t^\top \mathbf{\Sigma}_{i,in} \mathbf{\hat{B}}_t) \Big\|_2  +\frac{1}{n}\Big\|\sum_{i=1}^n \mathbf{\hat{B}}_t^\top \mathbf{\Sigma}_{i,in} \mathbf{\hat{B}}_\ast \mathbf{w}_{\ast,i} \mathbf{w}_{\ast,i}^\top  \mathbf{\hat{B}}_t \mathbf{\Sigma}_{i,in} \mathbf{\hat{B}}_\ast^\top \Big\|_2 \nonumber \\
   &\quad +\frac{1}{n}\Big\| \sum_{i=1}^n(\mathbf{I}_k - \mathbf{\hat{B}}_t^\top \mathbf{\Sigma}_{i,in} \mathbf{\hat{B}}_t)\mathbf{w}_t\mathbf{w}_{\ast,i}^\top  \mathbf{\hat{B}}_t \mathbf{\Sigma}_{i,in} \mathbf{\hat{B}}_\ast^\top + 
   \mathbf{\hat{B}}_t^\top \mathbf{\Sigma}_{i,in} \mathbf{\hat{B}}_\ast \mathbf{w}_{\ast,i}
   \mathbf{w}_t^\top (\mathbf{I}_k - \mathbf{\hat{B}}_t^\top \mathbf{\Sigma}_{i,in} \mathbf{\hat{B}}_t) 
   \Big\|_2^2  \label{tri0} \\
   &\leq L_{\max}^2 \max_{i\in [n]}\|\mathbf{I}_k - \mathbf{\hat{B}}_t^\top \mathbf{\Sigma}_{i,in} \mathbf{\hat{B}}_t\|_2^2 + L_{\max}^2 \max_{i\in [n]}\| \mathbf{\hat{B}}_t^\top \mathbf{\Sigma}_{i,in} \mathbf{\hat{B}}_\ast\|_2^2  \nonumber \\
   &\quad  + 2 L_{\max}^2 \max_{i\in [n]}\|\mathbf{I}_k - \mathbf{\hat{B}}_t^\top \mathbf{\Sigma}_{i,in} \mathbf{\hat{B}}_t\|_2 \| \mathbf{\hat{B}}_t^\top \mathbf{\Sigma}_{i,in} \mathbf{\hat{B}}_\ast\|_2  \label{tri1} \\
   &\leq L_{\max}^2 \delta_{in}^2 +  L_{\max}^2(1+\delta_{in})^2 +  2 L_{\max}^2\delta_{in}(1+\delta_{in}) \label{versh1} \\
   &= L_{\max}^2(2\delta_{in} + 1)^2 
%   \frac{2}{n} \left\|(\mathbf{I}_k - \mathbf{\hat{B}}_t^\top \mathbf{\Sigma}_{i,in} \mathbf{\hat{B}}_t)\mathbf{w}_t \mathbf{1}_n^\top\right\|_2^2 +  \frac{2}{n}\left\|\mathbf{\hat{B}}_t^\top \mathbf{\Sigma}_{i,in} \mathbf{\hat{B}}_\ast \mathbf{W}_{\ast}^\top \right\|_2^2 \nonumber \\
%   &\leq {2}L_\ast^2 \left\|\mathbf{I}_k - \mathbf{\hat{B}}_t^\top \mathbf{\Sigma}_{i,in} \mathbf{\hat{B}}_t\right\|_2^2 +  {2 L_\ast^2} \left\|\mathbf{\hat{B}}_t^\top \mathbf{\Sigma}_{i,in} \mathbf{\hat{B}}_\ast \right\|_2^2 \label{cs1} \\
%   &\leq 2c L_\ast^2 \frac{k+ 100 \log(n)}{m_{in}} + {2 L_\ast^2}\left\|\mathbf{\hat{B}}_t^\top \mathbf{\Sigma}_{i,in} \mathbf{\hat{B}}_\ast \right\|_2^2 \label{use_concen1}\\
%   &\leq 2c L_\ast^2 \frac{k+ 100 \log(n)}{m_{in}}+ {2} L_\ast^2 \left( 1 +  c\frac{k+ 100 \log(n)}{m_{in}}\right) \label{use_concen2} \\
%   &\leq {2} L_\ast^2 +  4c L_\ast^2 \frac{k+ 100 \log(n)}{m_{in}}
\end{align}
where \eqref{tri0} and \eqref{tri1} follow from the triangle inequality, and \eqref{versh1} follows from \eqref{concen1} and Theorem 4.6.1. in Vershynin with probability at least $1- 4n^{-99}$ after using a union bound over $i \in [n]$.
% from the Cauchy-Schwarz inequality, and \eqref{use_concen1} follows from \eqref{concen1} with probability at least $1- 2n^{-100}$, and \eqref{use_concen2} follows similarly from Theorem 4.6.1. in Vershynin with probability at least $1- 2n^{-100}$.


Similarly, we can show
\begin{align}
  \sigma_{\min} \left( \frac{1}{n} \sum_{i = 1}^n \mathbf{w}_{t,i}\mathbf{w}_{t,i}^\top\right) 
   &=  %\left\| \frac{1}{n}  \mathbf{W}_{t,in}^\top \mathbf{W}_{t,in}\right\|_2 \nonumber \\&= %\frac{1}{n}\left\|\mathbf{W}_{t,in}\right\|_2^2 \nonumber \\&= 
   \frac{1}{n}\sigma_{\min}\Big(\sum_{i=1}^n (\mathbf{I}_k - \mathbf{\hat{B}}_t^\top \mathbf{\Sigma}_{i,in} \mathbf{\hat{B}}_t)\mathbf{w}_t\mathbf{w}_t^\top (\mathbf{I}_k - \mathbf{\hat{B}}_t^\top \mathbf{\Sigma}_{i,in} \mathbf{\hat{B}}_t)  + \mathbf{\hat{B}}_t^\top \mathbf{\Sigma}_{i,in} \mathbf{\hat{B}}_\ast \mathbf{w}_{\ast,i} \mathbf{w}_{\ast,i}^\top  \mathbf{\hat{B}}_t \mathbf{\Sigma}_{i,in} \mathbf{\hat{B}}_\ast^\top  \nonumber \\
   &\quad + (\mathbf{I}_k - \mathbf{\hat{B}}_t^\top \mathbf{\Sigma}_{i,in} \mathbf{\hat{B}}_t)\mathbf{w}_t\mathbf{w}_{\ast,i}^\top  \mathbf{\hat{B}}_t \mathbf{\Sigma}_{i,in} \mathbf{\hat{B}}_\ast^\top + 
   \mathbf{\hat{B}}_t^\top \mathbf{\Sigma}_{i,in} \mathbf{\hat{B}}_\ast \mathbf{w}_{\ast,i}
   \mathbf{w}_t^\top (\mathbf{I}_k - \mathbf{\hat{B}}_t^\top \mathbf{\Sigma}_{i,in} \mathbf{\hat{B}}_t) 
   \Big) \nonumber  \\
   &= \frac{1}{n}\sigma_{\min}\Big(\sum_{i=1}^n (\mathbf{I}_k - \mathbf{\hat{B}}_t^\top \mathbf{\Sigma}_{i,in} \mathbf{\hat{B}}_t)\mathbf{w}_t\mathbf{w}_t^\top (\mathbf{I}_k - \mathbf{\hat{B}}_t^\top \mathbf{\Sigma}_{i,in} \mathbf{\hat{B}}_t)  + \mathbf{\hat{B}}_t^\top \mathbf{\Sigma}_{i,in} \mathbf{\hat{B}}_\ast \mathbf{w}_{\ast,i} \mathbf{w}_{\ast,i}^\top  \mathbf{\hat{B}}_\ast \mathbf{\Sigma}_{i,in} \mathbf{\hat{B}}_t^\top  \nonumber \\
   &\quad \quad \quad \quad \quad \quad + \mathbf{A}_i + \mathbf{A}_i^\top
   \Big) \nonumber  \\
   &\geq \frac{1}{n}\sigma_{\min}\Big(\sum_{i=1}^n (\mathbf{I}_k - \mathbf{\hat{B}}_t^\top \mathbf{\Sigma}_{i,in} \mathbf{\hat{B}}_t)\mathbf{w}_t\mathbf{w}_t^\top (\mathbf{I}_k - \mathbf{\hat{B}}_t^\top \mathbf{\Sigma}_{i,in} \mathbf{\hat{B}}_t)  + \mathbf{\hat{B}}_t^\top \mathbf{\Sigma}_{i,in} \mathbf{\hat{B}}_\ast \mathbf{w}_{\ast,i} \mathbf{w}_{\ast,i}^\top  \mathbf{\hat{B}}_\ast \mathbf{\Sigma}_{i,in} \mathbf{\hat{B}}_t^\top\Big) \nonumber \\
   &\quad \quad \quad \quad \quad \quad  - \frac{1}{n}\sigma_{\max}( \sum_{i=1}^n \mathbf{A}_i + \mathbf{A}_i^\top) \label{ab}  \\
   &\geq  \frac{1}{n}\sigma_{\min}\Big(\sum_{i=1}^n (\mathbf{I}_k - \mathbf{\hat{B}}_t^\top \mathbf{\Sigma}_{i,in} \mathbf{\hat{B}}_t)\mathbf{w}_t\mathbf{w}_t^\top (\mathbf{I}_k - \mathbf{\hat{B}}_t^\top \mathbf{\Sigma}_{i,in} \mathbf{\hat{B}}_t)\Big) \nonumber\\
   &\quad + \frac{1}{n}\sigma_{\min}\Big(\sum_{i=1}^n \mathbf{\hat{B}}_t^\top \mathbf{\Sigma}_{i,in} \mathbf{\hat{B}}_\ast \mathbf{w}_{\ast,i} \mathbf{w}_{\ast,i}^\top  \mathbf{\hat{B}}_\ast \mathbf{\Sigma}_{i,in} \mathbf{\hat{B}}_t^\top\Big) - \frac{2}{n}\sigma_{\max}( \sum_{i=1}^n \mathbf{A}_i) \label{ab2} \\
   &\geq \frac{1}{n}\sigma_{\min}\Big(\sum_{i=1}^n \mathbf{\hat{B}}_t^\top \mathbf{\Sigma}_{i,in} \mathbf{\hat{B}}_\ast \mathbf{w}_{\ast,i} \mathbf{w}_{\ast,i}^\top  \mathbf{\hat{B}}_\ast \mathbf{\Sigma}_{i,in} \mathbf{\hat{B}}_t^\top\Big) - {2}\max_{i\in [n]}\sigma_{\max}( \mathbf{A}_i) \\
   &\geq \frac{1}{n}\sigma_{\min}\Big(\sum_{i=1}^n \mathbf{\hat{B}}_t^\top \mathbf{\Sigma}_{i,in} \mathbf{\hat{B}}_\ast \mathbf{w}_{\ast,i} \mathbf{w}_{\ast,i}^\top  \mathbf{\hat{B}}_\ast \mathbf{\Sigma}_{i,in} \mathbf{\hat{B}}_t^\top\Big) - {2}\max_{i\in [n]}\sigma_{\max}( \mathbf{A}_i)
   \nonumber \\
   &\geq \frac{1}{n}\sigma_{\min}\Big(\sum_{i=1}^n \mathbf{\hat{B}}_t^\top \mathbf{\Sigma}_{i,in} \mathbf{\hat{B}}_\ast \mathbf{w}_{\ast,i} \mathbf{w}_{\ast,i}^\top  \mathbf{\hat{B}}_\ast \mathbf{\Sigma}_{i,in} \mathbf{\hat{B}}_t^\top\Big) -2 L_{\max}^2 \delta_{in}(1+\delta_{in})\label{versh1}
%   & ------------ \nonumber \\
%   & \frac{1}{n} \sigma_{\min}^2\left( (\mathbf{I}_k - \mathbf{\hat{B}}_t^\top \mathbf{\Sigma}_{i,in} \mathbf{\hat{B}}_t)\mathbf{w}_t \mathbf{1}_n^\top + \mathbf{\hat{B}}_t^\top \mathbf{\Sigma}_{i,in} \mathbf{\hat{B}}_\ast \mathbf{W}_{\ast}^\top  \right) \nonumber \\
%   &\geq \frac{1}{n}  \sigma_{\min}^2\left( \mathbf{\hat{B}}_t^\top \mathbf{\Sigma}_{i,in} \mathbf{\hat{B}}_\ast \mathbf{W}_{\ast}^\top  \right) - \frac{2}{n} \sigma_{\max}\left(  \mathbf{\hat{B}}_t^\top \mathbf{\Sigma}_{i,in} \mathbf{\hat{B}}_\ast \mathbf{W}_{\ast}^\top \right)  \sigma_{\max}\left( (\mathbf{I}_k - \mathbf{\hat{B}}_t^\top \mathbf{\Sigma}_{i,in} \mathbf{\hat{B}}_t)\mathbf{w}_t \mathbf{1}_n^\top\right)   \label{ab} \\
%   &\geq  \mu_\ast^2 \sigma_{\min}^2\left( \mathbf{\hat{B}}_t^\top \mathbf{\Sigma}_{i,in} \mathbf{\hat{B}}_\ast \right) - 2L_\ast^2 \sigma_{\max}\left(  \mathbf{\hat{B}}_t^\top \mathbf{\Sigma}_{i,in} \mathbf{\hat{B}}_\ast \right) \sigma_{\max}\left( \mathbf{I}_k - \mathbf{\hat{B}}_t^\top \mathbf{\Sigma}_{i,in} \mathbf{\hat{B}}_t\right)   \nonumber \\
%   &\geq \mu_\ast^2 \left(1 - c \frac{k+ 100 \log(n)}{m_{in}}\right) - 2L_\ast^2 \sqrt{c/2} \left(1 + \sqrt{c/2} \frac{\sqrt{k}+ 10 \sqrt{\log(n)}}{\sqrt{m_{in}}} \right) \frac{\sqrt{k}+ 10 \sqrt{\log(n)}}{\sqrt{m_{in}}} \label{versh1} \\
%   &= \mu_{\ast}^2 - 2c (L_\ast^2+ \mu_{\ast}^2) \frac{k+ 100 \log(n)}{m_{in}} - 2 L_\ast^2 \sqrt{c/2}  \frac{\sqrt{k}+ 10 \sqrt{\log(n)}}{\sqrt{m_{in}}} \\
%   &=: \mu^2
\end{align}
where $\mathbf{A}_i \coloneqq (\mathbf{I}_k - \mathbf{\hat{B}}_t^\top \mathbf{\Sigma}_{i,in} \mathbf{\hat{B}}_t)\mathbf{w}_t\mathbf{w}_{\ast,i}^\top  \mathbf{\hat{B}}_t \mathbf{\Sigma}_{i,in} \mathbf{\hat{B}}_\ast^\top$, 
\eqref{ab} follows from the fact that $\sigma_{\min}(\mathbf{C}_1 + \mathbf{C}_2) \geq \sigma_{\min}(\mathbf{C}_1) - \sigma_{\max}(\mathbf{C}_2)$, 
% thus $\sigma_{\min}^2(\mathbf{C}_1 + \mathbf{C}_2) \geq \sigma_{\min}^2(\mathbf{A}_1) - 2\sigma_{\min}(\mathbf{C}_1) \sigma_{\max}(\mathbf{C}_2) + \sigma_{\max}^2(\mathbf{C}_2) \geq \sigma_{\min}^2(\mathbf{C}_1) - 2\sigma_{\max}(\mathbf{C}_1) \sigma_{\max}(\mathbf{C}_2) $ 
for any two matrices $\mathbf{C}_1$ and $\mathbf{C}_2$, \eqref{ab2} follows from Weyl's inequality, and \eqref{versh1} follows from Theorem 4.6.1 in Vershynin with probability at least $1- 4 n^{-100}$. Next, note that 
\begin{align}
&\frac{1}{n}\sigma_{\min}\Big(\sum_{i=1}^n \mathbf{\hat{B}}_t^\top \mathbf{\Sigma}_{i,in} \mathbf{\hat{B}}_\ast \mathbf{w}_{\ast,i} \mathbf{w}_{\ast,i}^\top  \mathbf{\hat{B}}_t \mathbf{\Sigma}_{i,in} \mathbf{\hat{B}}_\ast^\top\Big) \nonumber \\
&= 
   \frac{1}{n} \sigma_{\min}\left(  \sum_{i=1}^n\mathbf{\hat{B}}_t^\top \mathbf{\hat{B}}_\ast\mathbf{w}_{\ast,i}\mathbf{w}_{\ast,i}^\top \mathbf{\hat{B}}_\ast^\top  \mathbf{\hat{B}}_t + \mathbf{\hat{B}}_t^\top (\mathbf{\Sigma}_{i,in} - \mathbf{I}_k)\mathbf{\hat{B}}_\ast\mathbf{w}_{\ast,i}\mathbf{w}_{\ast,i}^\top \mathbf{\hat{B}}_\ast^\top  \mathbf{\hat{B}}_t + \mathbf{\hat{B}}_t^\top \mathbf{\Sigma}_{i,in}\mathbf{\hat{B}}_\ast\mathbf{w}_{\ast,i}\mathbf{w}_{\ast,i}^\top \mathbf{\hat{B}}_\ast^\top (\mathbf{\Sigma}_{i,in} - \mathbf{I}_k) \mathbf{\hat{B}}_t \right)  \nonumber \\
   &\geq \frac{1}{n} \sigma_{\min}\left(  \sum_{i=1}^n\mathbf{\hat{B}}_t^\top \mathbf{\hat{B}}_\ast\mathbf{w}_{\ast,i}\mathbf{w}_{\ast,i}^\top \mathbf{\hat{B}}_\ast^\top  \mathbf{\hat{B}}_t\right) -\frac{1}{n}\sigma_{\max}\left(\sum_{i=1}^n \mathbf{\hat{B}}_t^\top (\mathbf{\Sigma}_{i,in} - \mathbf{I}_k)\mathbf{\hat{B}}_\ast\mathbf{w}_{\ast,i}\mathbf{w}_{\ast,i}^\top \mathbf{\hat{B}}_\ast^\top  \mathbf{\hat{B}}_t\right) \nonumber \\
   &\quad \quad - \frac{1}{n}\sigma_{\max}\left(\sum_{i=1}^n \mathbf{\hat{B}}_t^\top \mathbf{\Sigma}_{i,in}\mathbf{\hat{B}}_\ast\mathbf{w}_{\ast,i}\mathbf{w}_{\ast,i}^\top \mathbf{\hat{B}}_\ast^\top (\mathbf{\Sigma}_{i,in} - \mathbf{I}_k) \mathbf{\hat{B}}_t \right)  \nonumber \\
   &\geq \sigma_{\min}^2(\mathbf{\hat{B}}_t^\top  \mathbf{\hat{B}}_\ast) \sigma_{\min} \left( \frac{1}{n}\sum_{i=1}^n \mathbf{w}_{\ast,i}\mathbf{w}_{\ast,i}^\top\right) - L_{\max}^2 \max_{i\in [n]} \| \mathbf{\hat{B}}_t^\top (\mathbf{\Sigma}_{i,in} - \mathbf{I}_k)\mathbf{\hat{B}}_\ast\|_2 - L_{\max}^2  \max_{i\in [n]} \| \mathbf{\hat{B}}_t^\top (\mathbf{\Sigma}_{i,in} - \mathbf{I}_k)\mathbf{\hat{B}}_\ast\|_2 \| \mathbf{\hat{B}}_t^\top \mathbf{\Sigma}_{i,in}\mathbf{\hat{B}}_\ast\|_2 \nonumber \\
   &= \mu_\ast^2 E_0 - L_{\max}^2 (2\delta_{in} + \delta_{in}^2) 
\end{align}
Combining this with \eqref{versh1} completes the proof.

\end{proof}

\subsection{Infinite outer loop samples}
The following result shows contraction in the case $m_{in} = \Omega\left(\frac{L_\ast^4(k +\log(n))}{\mu_\ast^4 E_0^2}\right)$ and $m_{out} = \infty$.
\begin{lemma}
Suppose that there are infinite samples for the outer loop update, i.e. $m_{out} = \infty$ and $\mathbf{B}_{t+1}= \mathbf{\hat{B}}_t\left(\mathbf{I} - \frac{\beta}{n}\sum_{i=1}^n \mathbf{w}_{t,i}\mathbf{w}_{t,i}^\top\right) + \mathbf{\hat{B}}_\ast\left(\frac{\beta}{n} \sum_{i=1}^n \mathbf{w}_{\ast,i} \mathbf{w}_{t,i}^\top \right)$. Let $\delta_{in} \coloneqq c \frac{\sqrt{k} + 10\sqrt{\log(n)}}{\sqrt{m_{in}}}$ for some absolute constant $c$ and let $\beta \leq 1/(L_{\max}^2(2\delta_{in}+1)^2)$ and $\alpha=1$.
% Assume that $\sigma_{\min}\left(\frac{1}{n} \sum_{i=1}^n \mathbf{w}_{t,i}\mathbf{w}_{t,i}^\top \right)\geq \mu^2$,  $\sigma_{\min}\left(\frac{1}{n} \sum_{i=1}^n \mathbf{w}_{\ast,i}\mathbf{w}_{\ast,i}^\top \right) \geq \mu_\ast^2 $, \\
% $ \sigma_{\max}\left(\frac{1}{n} \sum_{i=1}^n \mathbf{w}_{t,i}\mathbf{w}_{t,i}^\top \right)\leq L^2$, and $\max_{i\in[n]} \|\mathbf{w}_{\ast,i}\|_2  \leq L_\ast$, and $\beta \leq 1/L^2$. Further assume that $\|\mathbf{w}_t\|_2 \leq 1$, and that $\|\mathbf{w}_{t,i} - \mathbf{\hat{B}}^\top_{t} \mathbf{\hat{B}}_\ast \mathbf{w}_{\ast,i}\|_2 \leq L_\ast \epsilon_i$. Define $\epsilon \coloneqq \sqrt{\frac{1}{{n}}\sum_{i=1}^n \epsilon_i^2}$.
Then with probability at least $1-4n^{-99}$,
\begin{align}
   \dist(\mathbf{\hat{B}}_{t+1}, \mathbf{\hat{B}}_\ast)&\leq \frac{1 - \beta \mu_\ast^2 E_0 + 4\beta L_{\max}^2(\delta_{in} + \delta_{in}^2)}{\sqrt{1 - 2 \beta \delta L_{\max}^2 (2\delta_{in} + 1)}}\dist(\mathbf{\hat{B}}_{t}, \mathbf{\hat{B}}_\ast) 
\end{align}
\end{lemma}
\begin{proof}
Note that 
    \begin{align}
       \mathbf{\hat{B}}_{\ast,\perp}^\top\mathbf{B}_{t+1} &= \mathbf{\hat{B}}_{\ast,\perp}^\top\mathbf{\hat{B}}_{t}\left(\mathbf{I} - \frac{\beta}{n}\sum_{i=1}^n \mathbf{w}_{t,i}\mathbf{w}_{t,i}^\top\right)
    \end{align}
    Let $\mathbf{\hat{B}}_{t+1}\mathbf{R}_{t+1} = \mathbf{B}_{t+1}$ be the QR decomposition of $\mathbf{B}_{t+1}$. Then we have 
    \begin{align}
        \dist(\mathbf{\hat{B}}_{t+1}, \mathbf{\hat{B}}_\ast) &\leq \dist(\mathbf{\hat{B}}_{t}, \mathbf{\hat{B}}_\ast) \left\|\mathbf{I} - \frac{\beta}{n}\sum_{i=1}^n \mathbf{w}_{t,i}\mathbf{w}_{t,i}^\top\right\|_2 \|\mathbf{R}_{t+1}^{-1}\|_2 \nonumber \\
        &\leq \dist(\mathbf{\hat{B}}_{t}, \mathbf{\hat{B}}_\ast) (1 - \beta \mu^2) \|\mathbf{R}_{t+1}^{-1}\|_2 \label{contract1} \\
        &\leq \dist(\mathbf{\hat{B}}_{t}, \mathbf{\hat{B}}_\ast) (1 - \beta \mu_\ast^2 E_0 + 4\beta L_{\max}^2(\delta_{in} + \delta_{in}^2) ) \|\mathbf{R}_{t+1}^{-1}\|_2 \label{use_lem_cond}
    \end{align}
    where \eqref{use_lem_cond} follows from Lemma \ref{lem:cond} with probability at least $1- 4n^{-99}$. 
    It remains to upper bound $\|\mathbf{R}_{t+1}^{-1}\|_2$.

% Again we have $\dist(\mathbf{\hat{B}}_{t+1}, \mathbf{\hat{B}}_\ast)\leq \dist(\mathbf{\hat{B}}_{t}, \mathbf{\hat{B}}_\ast) (1 - \beta \mu^2) \|\mathbf{R}_{t+1}^{-1}\|_2$. 
Let $\mathbf{e}_i \coloneqq  \mathbf{w}_{t,i} - \mathbf{\hat{B}}^\top_{t} \mathbf{\hat{B}}_\ast \mathbf{w}_{\ast,i}$. Observe that 
    \begin{align}
        \mathbf{R}_{t+1}^\top \mathbf{R}_{t+1} &= \mathbf{B}_{t+1}^\top \mathbf{B}_{t+1} \nonumber \\
        &= \mathbf{\hat{B}}_{t}^\top \mathbf{\hat{B}}_{t} - \frac{\beta}{n} \sum_{i=1}^n \left(\mathbf{\hat{B}}_{t}^\top \mathbf{\hat{B}}_t \mathbf{w}_{t,i} - \mathbf{\hat{B}}_{t}^\top \mathbf{\hat{B}}_\ast \mathbf{w}_{\ast,i}\right)\mathbf{w}_{t,i}^\top - \frac{\beta}{n} \sum_{i=1}^n \mathbf{w}_{t,i} \left( \mathbf{w}_{t,i}^\top \mathbf{\hat{B}}_t^\top \mathbf{\hat{B}}_t - \mathbf{w}_{\ast,i}^\top \mathbf{\hat{B}}_\ast^\top \mathbf{\hat{B}}_t \right) \nonumber \\
        &\quad + \left(\frac{\beta}{n} \sum_{i=1}^n \left(\mathbf{\hat{B}}_{t}^\top \mathbf{\hat{B}}_t \mathbf{w}_{t,i} - \mathbf{\hat{B}}_{t}^\top \mathbf{\hat{B}}_\ast \mathbf{w}_{\ast,i}\right)\mathbf{w}_{t,i}^\top\right)^\top \left(\frac{\beta}{n} \sum_{i=1}^n \left(\mathbf{\hat{B}}_{t}^\top \mathbf{\hat{B}}_t \mathbf{w}_{t,i} - \mathbf{\hat{B}}_{t}^\top \mathbf{\hat{B}}_\ast \mathbf{w}_{\ast,i}\right)\mathbf{w}_{t,i}^\top \right) \nonumber \\
    &= \mathbf{I}_{k} - \frac{\beta}{n} \sum_{i=1}^n \mathbf{e}_i\mathbf{w}_{t,i}^\top - \frac{\beta}{n} \sum_{i=1}^n \mathbf{w}_{t,i} \mathbf{e}_i^\top +\left(\frac{\beta}{n} \sum_{i=1}^n \mathbf{w}_{t,i} \mathbf{e}_i^\top \right) \left(\frac{\beta}{n} \sum_{i=1}^n \mathbf{e}_i \mathbf{w}_{t,i}^\top \right) 
    \end{align}
Next we use the fact that the $O(\beta^2)$ term is PSD, so we can drop it. 
Define $\mathbf{E} \in \mathbb{R}^{n \times k}$ as the matrix whose $i$-th row is $\mathbf{e}_i^\top$ and $\mathbf{W}_{t,in} \in \mathbb{R}^{n \times k}$ as the matrix whose $i$-th row is $\mathbf{w}_{t,i}^\top$.
We obtain
\begin{align}
\sigma_{\min}^2(\mathbf{R}_{t+1})&\geq 1 - 2 \beta \sigma_{\max}
\left( \frac{1}{n} \sum_{i=1}^n \mathbf{e}_i\mathbf{w}_{t,i}^\top  \right) \nonumber \\
% &\geq 1 - 2 \beta \max_{i \in [n]}
% \|\mathbf{e}_i\|_2 \|\mathbf{w}_{t,i}\|_2 \nonumber \\
&= 1 - 2 \beta \sigma_{\max}
\left( \frac{1}{n}  \mathbf{E}^\top \mathbf{W}_{t,in} \right) \nonumber \\
&\geq 1 - 2 \beta  \left\|\frac{1}{\sqrt{n}}\mathbf{E}\right\|_F \left\|\frac{1}{\sqrt{n}}\mathbf{W}_{t,in}\right\|_2 \nonumber \\
&\geq 1 - 2 \beta L_{\max}^2 \delta_{in} (2\delta_{in} + 1)
% &\geq 1 - 2 \beta  \epsilon L_\ast L
\end{align}
where the last inequality follows with probability at least $1-4n^{-99}$ from Lemmas \ref{lem:concen} and \ref{lem:cond}.
 So we have 
\begin{align}
    \dist(\mathbf{\hat{B}}_{t+1}, \mathbf{\hat{B}}_\ast)&\leq \frac{1 - \beta \mu_\ast^2 E_0 + 4\beta L_{\max}^2(\delta_{in} + \delta_{in}^2)}{\sqrt{1 - 2 \beta  L_{\max}^2 \delta_{in} (2\delta_{in} + 1)}}\dist(\mathbf{\hat{B}}_{t}, \mathbf{\hat{B}}_\ast) 
\end{align}
\end{proof}
% i don't think the union bounds can be removed

\textbf{The above result shows that $m_{in} = \Omega\left( \frac{L_{\max}^4 (k+\log(n))}{\mu_\ast^4 E_0^2}\right)$ results in linear convergence of the representation with high probability. Since $\mu_\ast^2= \Theta\left(\frac{1}{k}\right)$ and $L_{\max}^2 = \Theta(1)$, we essentially have $m_{in} = \Omega\left( \frac{k^2 (k+\log(n))}{E_0^2}\right)$.}

Why we cannot avoid union bound over tasks: intuitively, we need each task to concentrate individually. Concentration of the average across tasks is not enough. We will see that this is not the case for the outer loop update, which allows us to obtain a $\frac{1}{\sqrt{n}}$ factor in the concentration result.


\subsection{Finite Outer Loop Samples}
Now we consider the case in which we have finitely-many samples for the outer loop. Here the update for $\mathbf{B}$ is:
\begin{align}
    \mathbf{B}_{t+1} &= \mathbf{\hat{B}}_t  - \frac{\beta}{nm_{out}}\sum_{i=1}^n\sum_{j=1}^{m_{out}} \mathbf{x}_{i,j}\mathbf{x}_{i,j}^\top \mathbf{\hat{B}}_t  \mathbf{w}_{t,i}\mathbf{w}_{t,i}^\top + \frac{\beta}{n m_{out}} \sum_{i=1}^n \sum_{j=1}^{m_{out}} \mathbf{x}_{i,j}\mathbf{x}_{i,j}^\top \mathbf{\hat{B}}_\ast\mathbf{w}_{\ast,i} \mathbf{w}_{t,i}^\top  \nonumber \\
    &= \mathbf{\hat{B}}_t\left(\mathbf{I} - \frac{\beta}{n}\sum_{i=1}^n \mathbf{w}_{t,i}\mathbf{w}_{t,i}^\top\right) + \mathbf{\hat{B}}_\ast\left(\frac{\beta}{n} \sum_{i=1}^n \mathbf{w}_{\ast,i} \mathbf{w}_{t,i}^\top \right) \nonumber \\
    &\quad + \frac{\beta}{n} \sum_{i=1}^n \left(\mathbf{I}_d - \frac{1}{m_{out}}\sum_{j=1}^{m_{out}} \mathbf{x}_{i,j}\mathbf{x}_{i,j}^\top \right) \mathbf{\hat{B}}_t  \mathbf{w}_{t,i}\mathbf{w}_{t,i}^\top  - \frac{\beta}{n} \sum_{i=1}^n \left(\mathbf{I}_d - \frac{1}{m_{out}}\sum_{j=1}^{m_{out}} \mathbf{x}_{i,j}\mathbf{x}_{i,j}^\top \right) \mathbf{\hat{B}}_\ast \mathbf{w}_{\ast,i}\mathbf{w}_{t,i}^\top  
\end{align}
Therefore
\begin{align}
    \mathbf{\hat{B}}_{\ast,\perp}^\top \mathbf{B}_{t+1} &= \mathbf{\hat{B}}_{\ast,\perp}^\top\mathbf{\hat{B}}_t\left(\mathbf{I} - \frac{\beta}{n}\sum_{i=1}^n \mathbf{w}_{t,i}\mathbf{w}_{t,i}^\top\right) \nonumber \\
    &\quad + \frac{\beta}{n} \sum_{i=1}^n \mathbf{\hat{B}}_{\ast,\perp}^\top\left(\mathbf{I}_d - \frac{1}{m_{out}}\sum_{j=1}^{m_{out}} \mathbf{x}_{i,j}\mathbf{x}_{i,j}^\top \right)( \mathbf{\hat{B}}_t  \mathbf{w}_{t,i} - \mathbf{\hat{B}}_\ast \mathbf{w}_{\ast,i}) \mathbf{w}_{t,i}^\top % - \frac{\beta}{n} \sum_{i=1}^n \mathbf{\hat{B}}_{\ast,\perp}^\top\left(\mathbf{I}_d - \frac{1}{m_{out}}\sum_{j=1}^{m_{out}} \mathbf{x}_{i,j}\mathbf{x}_{i,j}^\top \right) \mathbf{\hat{B}}_\ast \mathbf{w}_{\ast,i}\mathbf{w}_{t,i}^\top  
\end{align}
Note that here we do not see a gain in the rate of concentration via multiplying the samples with their adjacent matrices, since $\mathbf{B}_{\ast,\perp}$ has $d-k$ columns, not $k$. So the naive outer loop sample complexity will grow with $d+\log(n)$ (using union bound). But we want $\frac{d}{n}$, otherwise we would be using many more samples than parameters. We would like to show that
\begin{align}
    \left\| \frac{1}{n} \sum_{i=1}^n \mathbf{\hat{B}}_{\ast,\perp}^\top\left(\mathbf{I}_d - \frac{1}{m_{out}}\sum_{j=1}^{m_{out}} \mathbf{x}_{i,j}\mathbf{x}_{i,j}^\top \right)( \mathbf{\hat{B}}_t  \mathbf{w}_{t,i} - \mathbf{\hat{B}}_\ast \mathbf{w}_{\ast,i})\mathbf{w}_{t,i}^\top  \right\|_2 &= O\left(\dist(\mathbf{\hat{B}}_t, \mathbf{\hat{B}}_\ast  )\sqrt{\frac{{d}}{{nm_{out}}}}\right) \label{goal1}
\end{align}
with high probability. Conditioning on $\mathbf{w}_{t,i}$, for any fixed unit vector $\mathbf{u} \in \mathbb{R}^k$,
$\mathbf{x}_{i,j}^\top (\mathbf{\hat{B}}_t  \mathbf{w}_{t,i}- \mathbf{\hat{B}}_\ast \mathbf{w}_{\ast,i})\mathbf{w}_{t,i}^\top \mathbf{u}$ is sub-Gaussian with sub-Gaussian norm $O(\|\mathbf{\hat{B}}_t  \mathbf{w}_{t,i}\mathbf{w}_{t,i}^\top- \mathbf{\hat{B}}_\ast \mathbf{w}_{\ast,i}\mathbf{w}_{t,i}^\top\|_2)$. Also, for any fixed unit vector $\mathbf{v} \in \mathbb{R}^{d-k}$, $\mathbf{v}^\top \mathbf{\hat{B}}_{\ast,\perp}^\top \mathbf{x}_{i,j}$ is sub-Gaussian with norm $O(1)$.

So using the variational definition of the spectral norm, we will obtain a sum of $n m_{out}$ independent sub-exponential random variables with norm $O(\|\mathbf{\hat{B}}_t  \mathbf{w}_{t,i}\mathbf{w}_{t,i}^\top- \mathbf{\hat{B}}_\ast \mathbf{w}_{\ast,i}\mathbf{w}_{t,i}^\top\|_2)$ and mean zero, so by Bernstein's inequality and a covering argument over $\mathcal{S}^{d-k-1}$ and $\mathcal{S}^{k-1}$ we can show \eqref{goal1} with $\dist(\mathbf{\hat{B}}_t, \mathbf{\hat{B}}_\ast)$ replaced by $\max_{i\in[n]}  \|\mathbf{\hat{B}}_t  \mathbf{w}_{t,i}\mathbf{w}_{t,i}^\top- \mathbf{\hat{B}}_\ast \mathbf{w}_{\ast,i}\mathbf{w}_{t,i}^\top\|_2$. 
In particular, conditioning on $\{\mathbf{w}_{t,i}\}_{i=1}^n$, we have 
\begin{align}
    \Bigg\| \frac{1}{n} \sum_{i=1}^n \mathbf{\hat{B}}_{\ast,\perp}^\top&\left(\mathbf{I}_d - \frac{1}{m_{out}}\sum_{j=1}^{m_{out}} \mathbf{x}_{i,j}\mathbf{x}_{i,j}^\top \right)( \mathbf{\hat{B}}_t  \mathbf{w}_{t,i} - \mathbf{\hat{B}}_\ast \mathbf{w}_{\ast,i})\mathbf{w}_{t,i}^\top  \Bigg\|_2 \nonumber \\
    &\leq c \max_{i\in[n]}  \|\mathbf{\hat{B}}_t  \mathbf{w}_{t,i}\mathbf{w}_{t,i}^\top- \mathbf{\hat{B}}_\ast \mathbf{w}_{\ast,i}\mathbf{w}_{t,i}^\top\|_2 \max \left( \frac{\sqrt{d}+ \lambda}{\sqrt{nm_{out}}}, \frac{(\sqrt{d}+ \lambda)^2}{nm_{out}} \right) \label{57}
\end{align}
for some absolute constant $c$, with probability at least $1 - 2 e^{-\lambda^2}$ over the outer loop samples. We will choose $\lambda= 10\sqrt{d}$ and let $\sqrt{nm_{out}} \geq 11\sqrt{d}$ to obtain
\begin{align}
    \Bigg\| \frac{1}{n} \sum_{i=1}^n \mathbf{\hat{B}}_{\ast,\perp}^\top&\left(\mathbf{I}_d - \frac{1}{m_{out}}\sum_{j=1}^{m_{out}} \mathbf{x}_{i,j}\mathbf{x}_{i,j}^\top \right)( \mathbf{\hat{B}}_t  \mathbf{w}_{t,i} - \mathbf{\hat{B}}_\ast \mathbf{w}_{\ast,i})\mathbf{w}_{t,i}^\top  \Bigg\|_2 \nonumber \\
    &\leq \max_{i\in[n]}  \|\mathbf{\hat{B}}_t  \mathbf{w}_{t,i}\mathbf{w}_{t,i}^\top- \mathbf{\hat{B}}_\ast \mathbf{w}_{\ast,i}\mathbf{w}_{t,i}^\top\|_2 \delta_{out}
\end{align}
with probability at least $1-2 e^{-100d}$, where $\delta_{out} \coloneqq \frac{11c\sqrt{d}}{\sqrt{nm_{out}}}$.
Now we must relate $ \max_{i\in [n]}\|\mathbf{\hat{B}}_t  \mathbf{w}_{t,i}\mathbf{w}_{t,i}^\top- \mathbf{\hat{B}}_\ast \mathbf{w}_{\ast,i}\mathbf{w}_{t,i}^\top\|_2$ and $\dist(\mathbf{\hat{B}}_t, \mathbf{\hat{B}}_\ast)$. Note that for any $i \in [n]$,
\begin{align}
    &\|\mathbf{\hat{B}}_t  \mathbf{w}_{t,i}\mathbf{w}_{t,i}^\top- \mathbf{\hat{B}}_\ast \mathbf{w}_{\ast,i}\mathbf{w}_{t,i}^\top\|_2 \nonumber \\
    &=\Big\|\mathbf{\hat{B}}_t \left( (\mathbf{I}- \mathbf{\hat{B}}_t^\top \mathbf{\Sigma}_{i,in} \mathbf{\hat{B}}_t)\mathbf{{w}}_t + \mathbf{\hat{B}}_t^\top \mathbf{\Sigma}_{i,in} \mathbf{\hat{B}}_\ast\mathbf{{w}}_{\ast,i} \right)  \left(\mathbf{{w}}_t^\top  (\mathbf{I}- \mathbf{\hat{B}}_t^\top \mathbf{\Sigma}_{i,in} \mathbf{\hat{B}}_t) + \mathbf{w}_{\ast,i}^\top \mathbf{\hat{B}}_\ast^\top \mathbf{\Sigma}_{i,in} \mathbf{\hat{B}}_t  \right) \nonumber \\
    &\quad \quad \quad \quad - \mathbf{\hat{B}}_\ast \mathbf{w}_{\ast,i}\left(\mathbf{{w}}_t^\top  (\mathbf{I}- \mathbf{\hat{B}}_t^\top \mathbf{\Sigma}_{i,in} \mathbf{\hat{B}}_t) + \mathbf{w}_{\ast,i}^\top \mathbf{\hat{B}}_\ast^\top \mathbf{\Sigma}_{i,in}\mathbf{\hat{B}}_t  \right) \Big\|_2 \nonumber \\
    &= \Big\|\mathbf{\hat{B}}_t (\mathbf{I}- \mathbf{\hat{B}}_t^\top \mathbf{\Sigma}_{i,in} \mathbf{\hat{B}}_t)\mathbf{{w}}_t\mathbf{{w}}_t^\top  (\mathbf{I}- \mathbf{\hat{B}}_t^\top \mathbf{\Sigma}_{i,in} \mathbf{\hat{B}}_t) + \mathbf{\hat{B}}_t (\mathbf{I}- \mathbf{\hat{B}}_t^\top \mathbf{\Sigma}_{i,in} \mathbf{\hat{B}}_t)\mathbf{{w}}_t\mathbf{{w}}_{\ast,i}^\top  \mathbf{\hat{B}}_\ast^\top \mathbf{\Sigma}_{i,in} \mathbf{\hat{B}}_t
    \nonumber \\
    &\quad \quad + \mathbf{\hat{B}}_t \mathbf{\hat{B}}_t^\top \mathbf{\Sigma}_{i,in} \mathbf{\hat{B}}_\ast \mathbf{{w}}_{\ast,i} \mathbf{{w}}_{t}^\top (\mathbf{I}_d - \mathbf{\hat{B}}_t^\top \mathbf{\Sigma}_{i,in} \mathbf{\hat{B}}_t) +  
    \mathbf{\hat{B}}_t \mathbf{\hat{B}}_t^\top \mathbf{\Sigma}_{i,in} \mathbf{\hat{B}}_\ast \mathbf{{w}}_{\ast,i} \mathbf{{w}}_{\ast,i}^\top \mathbf{\hat{B}}_{\ast,i}^\top \mathbf{\Sigma}_{i,in} \mathbf{\hat{B}}_t \nonumber \\
    &\quad \quad  - \mathbf{\hat{B}}_\ast \mathbf{w}_{\ast,i}\mathbf{{w}}_t^\top  (\mathbf{I}- \mathbf{\hat{B}}_t^\top \mathbf{\Sigma}_{i,in} \mathbf{\hat{B}}_t) - \mathbf{\hat{B}}_\ast \mathbf{w}_{\ast,i} \mathbf{w}_{\ast,i}^\top \mathbf{\hat{B}}_\ast^\top \mathbf{\Sigma}_{i,in}\mathbf{\hat{B}}_t   \Big\|_2 \nonumber \\    
    &\leq L_{\max}^2\|\mathbf{I}- \mathbf{\hat{B}}_t^\top \mathbf{\Sigma}_{i,in} \mathbf{\hat{B}}_t\|^2_2 + 2L_{\max}^2\|\mathbf{I}- \mathbf{\hat{B}}_t^\top \mathbf{\Sigma}_{i,in} \mathbf{\hat{B}}_t\|_2\| \mathbf{\hat{B}}_\ast^\top \mathbf{\Sigma}_{i,in}\mathbf{\hat{B}}_t \|_2  \nonumber \\
    &\quad + L_{\max}^2\|\mathbf{\hat{B}}_t \mathbf{\hat{B}}_t^\top \mathbf{\Sigma}_{i,in}\mathbf{B}_\ast - \mathbf{B}_\ast \|_2   \| \mathbf{\hat{B}}_\ast^\top \mathbf{\Sigma}_{i,in}\mathbf{\hat{B}}_t \|_2 + L_{\max}^2\|\mathbf{I}- \mathbf{\hat{B}}_t^\top \mathbf{\Sigma}_{i,in} \mathbf{\hat{B}}_t\|_2 
\end{align}
Note that 
\begin{align}
    &\|\mathbf{\hat{B}}_t \mathbf{\hat{B}}_t^\top \mathbf{\Sigma}_{i,in}\mathbf{\hat{B}}_\ast - \mathbf{\hat{B}}_\ast \|_2 \nonumber \\
    &= \|\mathbf{\hat{B}}_t (\mathbf{\hat{B}}_t^\top \mathbf{\Sigma}_{i,in} \mathbf{\hat{B}}_\ast - \mathbf{\hat{B}}_t^\top \mathbf{B}_\ast) + \mathbf{\hat{B}}_t\mathbf{\hat{B}}_t^\top  \mathbf{\hat{B}}_\ast - \mathbf{\hat{B}}_\ast \|_2 \nonumber \\
    &\leq \|\mathbf{\hat{B}}_t (\mathbf{\hat{B}}_t^\top \mathbf{\Sigma}_{i,in} \mathbf{\hat{B}}_\ast - \mathbf{\hat{B}}_t^\top \mathbf{\hat{B}}_\ast) \|_2 + \|\mathbf{\hat{B}}_t\mathbf{\hat{B}}_t^\top  \mathbf{\hat{B}}_\ast - \mathbf{\hat{B}}_\ast \|_2  \nonumber \\
    &\leq \|\mathbf{\hat{B}}_t^\top \mathbf{\Sigma}_{i,in} \mathbf{\hat{B}}_\ast - \mathbf{\hat{B}}_t^\top \mathbf{\hat{B}}_\ast\|_2 + \dist(\mathbf{\hat{B}}_t,\mathbf{\hat{B}}_\ast)
\end{align}
From earlier, we have that $\max_{i\in [n]} \|\mathbf{\hat{B}}_t^\top \mathbf{\Sigma}_{i,in} \mathbf{B}_\ast - \mathbf{\hat{B}}_t^\top \mathbf{\hat{B}}_\ast\|_2 \leq \delta_{in}$ and $\max_{i\in [n]} \|\mathbf{\hat{B}}_t^\top \mathbf{\Sigma}_{i,in} \mathbf{\hat{B}}_t - \mathbf{I}_d\|_2 \leq \delta_{in}$ with probability at least $1-4n^{-99}$. Thus we have
\begin{align}
    \max_{i \in [n]}\|\mathbf{\hat{B}}_t  \mathbf{w}_{t,i}\mathbf{w}_{t,i}^\top- \mathbf{\hat{B}}_\ast \mathbf{w}_{\ast,i}\mathbf{w}_{t,i}^\top\|_2 &\leq L_{\max}^2 (1+ \delta_{in}) \dist(\mathbf{\hat{B}}_t,\mathbf{\hat{B}}_\ast) + L_{\max}^2\delta^2 + 2L_{\max}^2 \delta_{in}(1+\delta_{in}) + L_{\max}^2 \delta_{in}(1+\delta_{in}) \nonumber \\
    &= L_{\max}^2 (1+ \delta_{in}) \dist(\mathbf{\hat{B}}_t,\mathbf{\hat{B}}_\ast) +4 L_{\max}^2 \delta_{in}^2 +  3 L_{\max}^2 \delta_{in}
\end{align}
with probability at least $1-4n^{-99}$, then using the fact that $\mathbb{P}(A) = \mathbb{P}(A|B)\mathbb{P}(B) + \mathbb{P}(A|B^c)\mathbb{P}(B^c)$, we have
\begin{align}
    \Bigg\| \frac{1}{n} \sum_{i=1}^n \mathbf{\hat{B}}_{\ast,\perp}^\top&\left(\mathbf{I}_d - \frac{1}{m_{out}}\sum_{j=1}^{m_{out}} \mathbf{x}_{i,j}\mathbf{x}_{i,j}^\top \right)( \mathbf{\hat{B}}_t  \mathbf{w}_{t,i} - \mathbf{\hat{B}}_\ast \mathbf{w}_{\ast,i})\mathbf{w}_{t,i}^\top  \Bigg\|_2 \nonumber \\
    &\leq  L_{\max}^2\left(  (1+ \delta_{in}) \dist(\mathbf{\hat{B}}_t,\mathbf{\hat{B}}_\ast) +4 \delta_{in}^2 +  3\delta_{in} \right) \delta_{out} \label{62}
\end{align}
with probability at least $1-4n^{-99}-2e^{-100d}$. So we do not have linear convergence. We instead have
\begin{align}
    \dist(\mathbf{\hat{B}}_{t+1}, \mathbf{\hat{B}}_\ast ) &\leq \left((1 - \beta \mu^2 + \beta L_{\max}^2 \delta_{out}(1+\delta_{in}))\dist(\mathbf{\hat{B}}_{t}, \mathbf{\hat{B}}_\ast) + 4\beta L_{\max}^2 \delta_{out}\delta_{in}^2+ 3\beta L_{\max}^2\delta_{out}\delta_{in})\right) \|\mathbf{R}^{-1}_{t+1}\|_2
\end{align}
where
\begin{align}
    \delta_{in} = O\left(\frac{\sqrt{k}+ \sqrt{\log(n)}}{\sqrt{m_{in}}}\right),\quad \delta_{out} = O\left(\frac{\sqrt{d}}{\sqrt{n m_{out}}}\right)
\end{align}
and 
\begin{align}
    \sigma_{\min}^2\left( \mathbf{R}_{t+1}\right) &= \sigma_{\min}^{2}(\mathbf{B}_{t+1,pop}) - 2\beta \sigma_{\max}\left(\frac{1}{n}\sum_{i=1}^n \mathbf{B}_{t+1,pop}^\top  \left(\mathbf{I}_d - \frac{1}{m_{out}}\sum_{j=1}^{m_{out}} \mathbf{x}_{i,j}\mathbf{x}_{i,j}^\top \right)( \mathbf{\hat{B}}_t  \mathbf{w}_{t,i} - \mathbf{\hat{B}}_\ast \mathbf{w}_{\ast,i}) \mathbf{w}_{t,i}^\top  \right) \nonumber \\
    &\quad + \beta^2 \sigma_{\min}^2\left( \frac{1}{n}\sum_{i=1}^n  \left(\mathbf{I}_d - \frac{1}{m_{out}}\sum_{j=1}^{m_{out}} \mathbf{x}_{i,j}\mathbf{x}_{i,j}^\top \right)( \mathbf{\hat{B}}_t  \mathbf{w}_{t,i} - \mathbf{\hat{B}}_\ast \mathbf{w}_{\ast,i}) \mathbf{w}_{t,i}^\top  \right) \nonumber \\
    &\geq 1 - 2 \beta L_{\max}^2\delta_{in} (2\delta_{in}+1) - 2\beta \sigma_{\max}\left(\frac{1}{n}\sum_{i=1}^n \mathbf{B}_{t+1,pop}^\top  \left(\mathbf{I}_d - \frac{1}{m_{out}}\sum_{j=1}^{m_{out}} \mathbf{x}_{i,j}\mathbf{x}_{i,j}^\top \right)( \mathbf{\hat{B}}_t  \mathbf{w}_{t,i} - \mathbf{\hat{B}}_\ast \mathbf{w}_{\ast,i}) \mathbf{w}_{t,i}^\top  \right)
\end{align}
where $\mathbf{B}_{t+1,pop}= \mathbf{\hat{B}}_t\left(\mathbf{I} - \frac{\beta}{n}\sum_{i=1}^n \mathbf{w}_{t,i}\mathbf{w}_{t,i}^\top\right) + \mathbf{\hat{B}}_\ast\left(\frac{\beta}{n} \sum_{i=1}^n \mathbf{w}_{\ast,i} \mathbf{w}_{t,i}^\top \right)$ from the infinite-outer loop sample case.
Note that we can use the analysis from equations \eqref{57} thru \eqref{62} with $\mathbf{\hat{B}}_{\ast,\perp}$ replaced by $\mathbf{B}_{t+1,pop}$ to obtain
\begin{align}
    &\sigma_{\max}\left(\frac{1}{n}\sum_{i=1}^n \mathbf{B}_{t+1,pop}^\top  \left(\mathbf{I}_d - \frac{1}{m_{out}}\sum_{j=1}^{m_{out}} \mathbf{x}_{i,j}\mathbf{x}_{i,j}^\top \right)( \mathbf{\hat{B}}_t  \mathbf{w}_{t,i} - \mathbf{\hat{B}}_\ast \mathbf{w}_{\ast,i}) \mathbf{w}_{t,i}^\top  \right) \nonumber \\
    &\leq L_{\max}^2\left((1+\delta_{in})\dist(\mathbf{\hat{B}}_t, \mathbf{\hat{B}}_\ast) + 4\delta_{in}^2 +3\delta_{in} \right) \delta_{out}' \|\mathbf{B}_{t+1,pop}\|_2 \nonumber \\
    &\leq  L_{\max}^2 (1+2\delta_{in})^2 \delta_{out}' \|\mathbf{B}_{t+1,pop}\|_2  \nonumber \\
    &=   L_{\max}^2 (1+2\delta_{in})^2 \delta_{out}' \left\|\mathbf{\hat{B}}_t\left(\mathbf{I} - \frac{\beta}{n}\sum_{i=1}^n \mathbf{w}_{t,i}\mathbf{w}_{t,i}^\top\right) + \mathbf{\hat{B}}_\ast\left(\frac{\beta}{n} \sum_{i=1}^n \mathbf{w}_{\ast,i} \mathbf{w}_{t,i}^\top \right)\right\|_2  \nonumber \\
    &\leq L_{\max}^2(1+2\delta_{in})^2 \delta_{out}'\left( \left\|\mathbf{I} - \frac{\beta}{n}\sum_{i=1}^n \mathbf{w}_{t,i}\mathbf{w}_{t,i}^\top\right\|_2 + \left\|\frac{\beta}{n} \sum_{i=1}^n \mathbf{w}_{\ast,i} \mathbf{w}_{t,i}^\top \right\|_2 \right) \nonumber \\
    &\leq L_{\max}^2(1+2\delta_{in})^2 \delta_{out}' \left( 1 - \beta \mu^2 + \beta L_\ast L \right) 
\end{align}
with probability at least $1- 4n^{-99} - 2e^{-100k}$, where $\delta_{out}' \coloneqq c\frac{\sqrt{k}}{\sqrt{nm_{out}}}$.
Putting everything together, we obtain the following result.


\begin{theorem}
Let $\delta_{in} = O\left( \frac{\sqrt{k} + 10\sqrt{\log(n)}}{\sqrt{m_{in}}}\right)$, $\delta_{out} = O\left( \frac{\sqrt{d}}{\sqrt{n m_{out}}}\right)$, and $\delta_{out}' = O\left( \frac{\sqrt{k}}{\sqrt{n m_{out}}}\right)$. Choose $\beta \leq 1/(L_{\max}^2(2\delta_{in}+1)^2)$ and $\alpha=1$. Then
\begin{align}
    \dist(\mathbf{\hat{B}}_{t+1}, \mathbf{\hat{B}}_\ast ) &\leq \frac{1 - \beta E_0\mu_\ast^2 + 4\beta L_{\max}^2 (\delta_{in}+\delta_{in}^2) ) + \beta L_{\max}^2 \delta_{out}(1+\delta_{in})}{\sqrt{1 - 2 \beta L_{\max}^2 \delta_{in} (1+2\delta_{in}) - 2\beta \delta_{out}'(1+2\delta_{in})^2  L_{\max}^2 \left( 1 - \beta \mu^2 + \beta L_{\max} L \right) }}\dist(\mathbf{\hat{B}}_{t}, \mathbf{\hat{B}}_\ast) \nonumber \\
    &\quad + \frac{2\beta L_{\max}^2 \delta_{out}\delta_{in} (1+ \delta_{in})}{\sqrt{1 - 2 \beta\delta_{in} L_{\max}^2 (1+2\delta_{in}) - 2\beta L_{\max}^2  \delta_{out}' (1+2\delta_{in})^2  \left( 1 - \beta \mu^2 + \beta L_{\max}L \right) }},
\end{align}
where $L \leq \sqrt{  L_{\max}^2 (2\delta_{in}+1)^2}$ and $\mu^2 \geq \mu_\ast^2 E_0 - 4 L_{\max}^2 (\delta_{in} + \delta_{in}^2)$, all
with probability at least $1- 4n^{-99} - 2e^{-100k} - 2e^{-100d}$. 
\end{theorem}
